# Supplementary material for: Drug Resistance Predictions Based on a Directed Flag Transformer
Source: arXiv:2403.02603 source file (2025-01-16)
Supplement: Supplementary file 1 [file SI_combine_flag.pdf]

# Supporting Information: Drug Resistance Predictions Based on a Directed Flag Transformer

Dong Chen,[†] Gengzhuo Liu,[†] Hongyan Du,[†] Benjamin Jones,[†] Junjie Wee,[†] Rui Wang,[‡] Jiahui Chen,[¶] Jana Shen,[*,§] and Guo-Wei Wei[*,‖]

† *Department of Mathematics, Michigan State University, MI, 48824, USA*

‡ *Simons Center for Computational Physical Chemistry, New York University, New York, NY, 10003*

¶ *Department of Mathematical Sciences, University of Arkansas, Fayetteville, AR 72701*

§ *Department of Pharmaceutical Sciences, University of Maryland School of Pharmacy, Baltimore, MD 21201*

‖ *Department of Mathematics & Department of Electrical and Computer Engineering & Department of Biochemistry and Molecular Biology, Michigan State University, MI, 48824, USA*

E-mail: Jana.Shen@rx.umaryland.edu; weig@msu.edu

# Table of Contents


- Supplementary Tables
- Supplementary Figures
- Supplementary Mathematical Methods
- Supplementary Computational Methods and Protocols
- Supplementary Notes

# Supplementary Tables

Table S1: Experimental data of SARS-CoV/CoV-2 Mpro-ligand complexes (part I)

| PDB | Proteins | Ligand | IC50(nM) | Ki(nM) | p$K_i$ | Ref. |
|---|---|---|---|---|---|---|
| 7SI9 | SARS-CoV-2 Mpro | 4WI | 26.03 | 1.88 | 8.726 | S1 |
| 8D4K | SARS-CoV-2 Mpro H172Y | K36 | 449.2 | 432.5 | 6.364 | S1 |
| 8D4M | SARS-CoV-2 Mpro S144A | K36 | 139.8 | 65.01 | 7.187 | S1 |
| 8DD1 | SARS-CoV-2 Mpro H164N | K36 | 126.3 | 37.95 | 7.421 | S1 |
| 8DD9 | SARS-CoV-2 Mpro S144L | K36 | 1812 | 1847 | 5.734 | S1 |
| 8DGB | SARS-CoV-2 Mpro Q192T | K36 | 237.2 | 119.7 | 6.922 | S1 |
| 6WTT | SARS-CoV-2 Mpro | B1S | 40.25 | 15.5 | 7.810 | S1 |
| 6XHM | SARS-CoV-2 Mpro | V2M | | 0.27 | 9.569 | S2 |
| 6XHL | SARS-CoV Mpro | V2M | | 4 | 8.398 | S2 |
| 6XHN | SARS-CoV Mpro | V3D | 15 | 5.38 | 8.269 | S2 |
| 2ZU4 | SARS-CoV Mpro | ZU3 | | 38 | 7.420 | S3 |
| 2ZU5 | SARS-CoV Mpro | ZU5 | | 400 | 6.398 | S3 |
| 6M0K | SARS-CoV-2 Mpro | FJC | 40 | | 7.398 | S4 |
| 6LZE | SARS-CoV-2 Mpro | FHR | 53 | | 7.276 | S4 |
| 2Z94 | SARS-CoV Mpro | TLD | | 1400 | 5.854 | S5 |
| 2Z9K | SARS-CoV Mpro | DOZ | | 320 | 6.495 | S5 |
| 2GX4 | SARS-CoV Mpro | NOL | | 53 | 7.276 | S6 |
| 5N5O | SARS-CoV Mpro | 8O5 | 240 | | 6.620 | S7 |
| 2GZ7 | SARS-CoV Mpro | D3F | 300 | | 6.523 | S8 |
| 2GZ8 | SARS-CoV Mpro | F3F | 3000 | | 5.523 | S8 |
| 6WTK | SARS-CoV-2 Mpro | UED | 400 | 171.4 | 6.766 | S9 |
| 6WTJ | SARS-CoV-2 Mpro | K36 | 190 | 81.42 | 7.089 | S9 |
| 3D62 | SARS-CoV Mpro | 959 | | 400 | 6.398 | S10 |
| 6XMK | SARS-CoV-2 Mpro | QYS | 450 | | 6.347 | S11 |
| 6W2A | SARS-CoV Mpro | QYS | 1100 | | 5.959 | S11 |
| 6XFN | SARS-CoV-2 Mpro | GOL | 450 | | 6.347 | S12 |
| 6LNY | SARS-CoV Mpro | EOC | 508 | 90.5 | 7.043 | S13 |
| 6Y2G | SARS-CoV-2 Mpro | O6K | 670 | 900 | 6.046 | S14 |
| 6M2N | SARS-CoV-2 Mpro | 3WL | 940 | | 6.027 | S15 |
| 6XA4 | SARS-CoV-2 Mpro | GOL | 0.41 | 0.6 | 9.222 | S12 |
| 2V6N | SARS-CoV Mpro | MES | | 1380 | 5.860 | S16 |
| 2Z94 | SARS-CoV Mpro | TLD | | 1400 | 5.854 | S5 |
| 5N19 | SARS-CoV Mpro | D03 | 1950 | | 5.710 | S7 |
| 2OP9 | SARS-CoV Mpro | WR1 | | 2200 | 5.658 | S17 |
| 3SN8 | SARS-CoV Mpro | S89 | | 8270 | 5.082 | S18 |
| 2GZ8 | SARS-CoV Mpro | F3F | 3000 | | 5.523 | S8 |
| 4MDS | SARS-CoV Mpro | 23H | 6200 | | 5.208 | S19 |
| 2AMD | SARS-CoV Mpro | 91N | | 6700 | 5.174 | S20 |
| 3SNE | SARS-CoV Mpro | MES | | 2240 | 5.650 | S18 |
| 1WOF | SARS-CoV Mpro | I12 | | 10700 | 4.971 | S20 |
| 3VB6 | SARS-CoV Mpro | EDO | 39000 | | 4.409 | S21 |
| 3SNC | SARS-CoV Mpro | DMS | | 72730 | 4.138 | S18 |
| 3VB4 | SARS-CoV Mpro | GOL | 49000 | | 4.310 | S21 |
| 3VB7 | SARS-CoV Mpro | GOL | 49000 | | 4.310 | S21 |
| 4TWW | SARS-CoV Mpro | 3A7 | 63000 | | 4.201 | S22 |
| 2ALV | SARS-CoV Mpro | CY6 | 70000 | | 4.155 | S23 |
| 2QIQ | SARS-CoV Mpro | CYV | 80000 | | 4.097 | S24 |
| 4TWY | SARS-CoV Mpro | 3BL | 108000 | | 3.967 | S22 |

p$K_i$ is calculated as $log_{10}(1/Ki)$ or $log_{10}(1/IC50)$ when $K_i$ data are unavailable.

Table S2: Experimental data on SARS-CoV/CoV-2 Mpro-ligand complexes (part II) taken from Ref. Nguyen et al.[S25]

| Complexes | logKa | Complexes | logKa | Complexes | p$K_i$ |
|---|---|---|---|---|---|
| 6y2g | 6.174 | narlaprevir | 5.245 | review-com12_6c | 6.301 |
| 6m2n | 6.027 | CHEMBL50 | 4.621 | CHEMBL1929017 | 5.245 |
| 7brp | 5.380 | CHEMBL2311733 | 4.350 | CHEMBL3402617 | 4.166 |
| 6wtk | 6.400 | review-com8-2s | 5.538 | review-com11_5b | 5.770 |
| 6wtj | 6.720 | CHEMBL2442075 | 4.650 | CHEMBL380403 | 4.922 |
| 6m0k | 7.420 | CHEMBL538957 | 4.306 | CHEMBL2402683 | 6.073 |
| 6lze | 7.280 | CHEMBL2402681 | 5.809 | CHEMBL208908 | 4.445 |
| 6lo0 | 6.080 | review-com11_5p | 6.921 | CHEMBL551569 | 3.939 |
| 6lny | 6.290 | CHEMBL2402499 | 5.230 | review-com46_45 | 3.757 |
| 5n19 | 5.710 | review3-com13-7 | 3.699 | 6y2g_13a | 5.619 |
| 2gx4 | 7.280 | CHEMBL213543 | 6.184 | review-com12_6b | 6.155 |
| 2amd | 5.710 | CHEMBL2311730 | 5.003 | review-com13_11u | 5.896 |
| 1wof | 4.910 | 6lnq-12b | 6.734 | CHEMBL557699 | 3.800 |
| 6wtt | 7.520 | review-com13_11t | 5.842 | review-com8-2t | 5.824 |
| CHEMBL2402500 | 4.636 | CHEMBL2402502 | 5.795 | review3-com145_17 | 4.551 |
| CHEMBL4130313 | 5.171 | review-com8-2i | 8.387 | review-com8-2r | 5.469 |
| CHEMBL2402676 | 5.135 | CHEMBL397154 | 5.003 | CHEMBL3402615 | 3.873 |
| CHEMBL2311700 | 4.408 | review-com11_5o | 6.097 | CHEMBL2402678 | 6.154 |
| CHEMBL2311729 | 4.122 | review-com11_5h | 8.201 | CHEMBL2402677 | 6.162 |
| review-com8-2m | 6.125 | CHEMBL2442077 | 5.164 | review-com11_5j | 7.523 |
| review-com9_10-25f | 4.538 | review-com11_5l | 5.174 | CHEMBL2402501 | 6.338 |
| CHEMBL235873 | 4.827 | review3-com55-3 | 3.073 | CHEMBL3402616 | 3.873 |
| CHEMBL1230135 | 5.047 | review-com11_5n | 7.658 | CHEMBL212080 | 7.240 |
| CHEMBL2402680 | 6.250 | review-com13_11s | 6.620 | CHEMBL2442082 | 5.208 |
| CHEMBL378188 | 4.093 | review-com8-2k | 7.854 | CHEMBL551181 | 3.235 |
| CHEMBL555220 | 4.467 | review-com8-2o | 6.187 | review-com11_5k | 7.585 |
| PSI | 4.981 | review3-com5 | 4.886 | CHEMBL4299306 | 6.748 |
| review-com54_30 | 4.620 | CHEMBL2316337 | 5.340 | CHEMBL2442076 | 5.384 |
| CHEMBL539208 | 3.440 | CHEMBL2311726 | 4.328 | CHEMBL1929018 | 6.411 |
| review-com13_11n | 6.481 | review-com13_11q | 5.203 | review-com8-2u | 5.125 |
| CHEMBL477164 | 6.697 | CHEMBL2402684 | 5.494 | CHEMBL1405735 | 5.655 |
| review-com11_5e | 6.796 | review3-com61_5b | 4.699 | CHEMBL1929021 | 5.003 |
| CHEMBL151 | 4.702 | CHEMBL406516 | 5.003 | review-com13_11p | 4.971 |
| CHEMBL2311705 | 4.298 | review-com9_10-26k | 6.076 | CHEMBL2311709 | 5.223 |
| CHEMBL2402507 | 5.494 | CHEMBL553172 | 3.873 | 6lnq-12a | 6.162 |
| PMC2597651_4 | 6.294 | PMC2597651_3 | 6.418 | CHEMBL2401746 | 6.213 |
| review-com13_11o | 5.071 | review-com8-2p | 8.523 | CHEMBL549695 | 6.220 |
| 6y2g_11r | 6.748 | CHEMBL2442079 | 5.113 | review3-com4 | 4.409 |
| CHEMBL2402508 | 6.374 | CHEMBL3402619 | 4.247 | review-com8-2n | 7.959 |
| CHEMBL2442074 | 5.039 | CalpainXII | 6.345 | CHEMBL537916 | 3.528 |
| review-com8-2l | 5.721 | review-com11_5c | 7.187 | review-com11_5r | 6.167 |
| review-com11_5g | 6.481 | CHEMBL2311731 | 5.259 | CHEMBL1929022 | 6.470 |
| CHEMBL2402682 | 5.076 | CHEMBL12798 | 3.682 | review3-com145_16r | 5.824 |
| review-com11_5a | 5.569 | calpeptin | 4.973 | CHEMBL63354 | 4.856 |
| review-com8-2j | 7.658 | CHEMBL1929015 | 4.210 | MG-132 | 5.406 |
| CHEMBL2402685 | 6.411 | CHEMBL28 | 3.550 | review-com11_5d | 7.174 |
| review3-com13-3 | 4.097 | review3-com61_5a | 4.824 | CHEMBL2402686 | 6.484 |
| CHEMBL377324 | 4.518 | CHEMBL2316336 | 4.408 | CHEMBL1929020 | 6.572 |
| review-com11_5i | 7.319 | CHEMBL2442073 | 5.421 | review-com54_2 | 6.222 |
| CHEMBL2402503 | 5.765 | CHEMBL2311727 | 5.281 | CHEMBL555061 | 4.680 |
| CHEMBL2402504 | 4.540 | CHEMBL2402692 | 6.184 | CHEMBL277716 | 5.648 |
| review-com54_33 | 4.620 | MG-115 | 5.501 | | |

Table S3: Five-fold cross-validation performance of the DFFormer-seq model on the SARS-CoV-2/CoV Mpro dataset.

| **Fold** | **1** | **2** | **3** | **4** | **5** | **Mean**$^a$ | **Mean**$^b$ |
|---|---|---|---|---|---|---|---|
| **PCC** | 0.642 | 0.597 | 0.570 | 0.735 | 0.723 | 0.654 | 0.644 |
| **RMSE** | 1.382 | 1.381 | 1.326 | 1.189 | 1.042 | 1.264 | 1.273 |

The RMSEs are given in kcal/mol. Mean$^a$ gives the average performance across five folds. Mean$^b$ means the performance on all predictions combined.

Table S4: Predicted binding affinity (BA) changes (10 × kcal/mol) due to single-point mutations at 19 binding site residues as well as P132 (the Omicron variant mutation site)

| Residue | A | R | N | D | C | Q | E | G | H | I |
|---|---|---|---|---|---|---|---|---|---|---|
| M49 | -7.4e-1 | -2.3e-2 | -8.1e-1 | -1.4 | -1.2 | -6.4e-1 | -9.9e-1 | -1.1e-1 | -7.1e-2 | -4.8e-1 |
| Y54 | 1.2 | -1.2 | 1.4 | 1.0 | 4.9e-1 | 8.4e-1 | 1.2 | 4.7e-1 | 1.6 | 1.6 |
| F140 | -7.1e-1 | -1.4 | -1.6 | -3.1 | -3.8e-1 | -1.5 | -2.8 | -4.6e-1 | -1.3 | -1.3 |
| L141 | 5.9e-1 | -6.1e-1 | 2.1e-1 | -7.5e-1 | -3.2e-1 | 4.6e-1 | 3.5e-1 | -4.2e-05 | 6.8e-1 | 2.5e-1 |
| N142 | 1.1 | -2.1 | n/a | -1.3 | -1.6 | 6.0e-1 | 9.4e-2 | -2.4 | 8.2e-1 | 3.9e-1 |
| G143 | -1.0 | -1.2 | -2.0 | -2.4 | -4.2e-1 | -2.4e-1 | -1.4 | n/a | -8.5e-1 | -3.8e-1 |
| S144 | 7.8e-1 | -2.0 | -1.5 | -1.8 | -3.4 | -2.5 | -3.7 | -4.2e-1 | -1.2 | -1.4 |
| H163 | 1.8e-1 | 7.2e-1 | -5.7e-1 | -1.4 | -1.9 | -7.8e-1 | -1.5 | -9.3e-1 | n/a | -1.2e-1 |
| H164 | 5.6e-1 | 1.7e-1 | 1.6 | -2.1e-1 | -3.7e-1 | -5.7e-1 | -2.0e-1 | -1.7 | n/a | 8.3e-1 |
| M165 | -2.7 | -2.9 | -3.3 | -2.2 | -2.0 | -2.2 | -2.5 | -4.7 | -1.4 | 2.8 |
| E166 | -2.6e-2 | 7.3e-1 | 6.4e-1 | -1.3 | 3.7e-1 | -1.5e-1 | n/a | 6.4e-1 | 1.9 | 2.2 |
| L167 | 1.8e-2 | -2.0 | -2.3 | -1.4 | -7.1e-1 | -2.8 | -1.6 | -9.1e-1 | -1.2 | -4.0e-1 |
| P168 | 8.1e-1 | 1.9e-1 | 4.2e-1 | 4.2e-1 | 2.4 | 2.7e-1 | 6.7e-1 | 1.0 | 6.0e-1 | 1.3 |
| H172 | -3.7e-1 | 6.1e-1 | 2.3e-1 | -1.6 | -1.1 | 1.6e-1 | -3.8e-1 | -1.3 | n/a | 1.8 |
| D187 | -3.3e-1 | -8.0e-1 | 8.1e-1 | n/a | -4.3e-2 | 1.2 | -3.5e-1 | 3.6e-1 | 9.4e-1 | 1.3 |
| R188 | -4.4e-1 | n/a | 6.6e-1 | 1.4e-1 | -2.8 | -1.6e-1 | 5.1e-2 | -8.2e-2 | 9.3e-1 | 6.8e-1 |
| Q189 | -1.2 | -7.0e-2 | 2.8e-1 | 1.1 | -7.5e-1 | n/a | -2.4e-1 | -2.5 | 1.0 | 3.4e-1 |
| T190 | -1.6 | 8.6e-1 | 1.2 | 9.8e-1 | 1.9 | 4.9e-1 | 3.6e-1 | -9.9e-1 | 2.5 | 1.0 |
| Q192 | 5.8e-1 | 8.3e-1 | 2.1e-1 | 1.1 | 3.4 | n/a | 5.4e-1 | -1.6e-1 | 1.6 | 1.6 |
| **P132** | 6.4e-1 | 4.2e-1 | 1.1 | 4.4e-1 | -2.4e-1 | 1.3 | 3.9e-1 | -6.5e-1 | 1.8 | -4.9e-1 |

| Residue | L | K | M | F | P | S | T | W | Y | V |
|---|---|---|---|---|---|---|---|---|---|---|
| M49 | -1.6 | -3.2e-1 | n/a | 6.7e-1 | -1.6 | -2.9e-1 | -1.6 | 3.4e-1 | 5.7e-1 | -5.5e-1 |
| Y54 | -1.5e-1 | 1.2 | 2.2 | 1.9 | 6.2e-1 | 1.2 | 5.6e-1 | 1.7 | n/a | 1.7 |
| F140 | -1.4 | -4.8e-1 | -4.8e-1 | n/a | -2.6 | -1.0 | -6.4e-1 | 1.9e-1 | -1.1 | 2.4e-1 |
| L141 | n/a | -4.3e-2 | 2.0 | 6.8e-1 | -1.4 | 1.4e-1 | -7.2e-1 | 4.3e-1 | -5.6e-1 | 6.4e-2 |
| N142 | -2.4e-1 | -8.2e-1 | 1.6 | -3.7e-2 | -1.1 | 4.1e-1 | -1.5 | -1.7 | 1.4e-1 | 5.1e-1 |
| G143 | -7.4e-1 | -6.8e-1 | 3.9e-1 | -1.0 | -1.0 | -1.3 | -1.5 | -4.4e-1 | -5.0e-2 | -7.1e-1 |
| S144 | -5.3 | -1.7 | -3.1 | -3.0 | -4.4 | n/a | -9.6e-1 | -1.3 | -2.0 | -1.4 |
| H163 | -1.7e-2 | 7.4e-1 | -8.1e-2 | 5.4e-1 | -1.1 | -8.9e-1 | -4.7e-1 | -1.4e-1 | 1.1 | -3.8e-1 |
| H164 | 6.0e-2 | 5.5e-1 | -3.7e-1 | 8.2e-1 | -6.5e-1 | 1.5e-2 | -4.3e-1 | 4.5e-1 | -1.3 | 8.2e-1 |
| M165 | 2.7 | -2.8 | n/a | 4.9 | -4.0 | -3.4 | -2.0 | -9.5e-1 | -4.2 | 7.4e-1 |
| E166 | 1.4 | 1.7 | 1.5 | 4.3 | 1.5 | -2.5e-1 | 2.9 | 4.3 | 3.4 | 2.2 |
| L167 | n/a | -2.6 | 1.7 | 1.1 | -1.2 | -1.0 | -1.1 | 2.4 | -2.7e-1 | -9.0e-2 |
| P168 | 7.4e-1 | 1.2 | 2.3 | 1.3 | n/a | 1.2 | 1.1 | 1.8e-1 | 5.6e-1 | 1.5 |
| H172 | -1.8e-1 | 5.2e-1 | 1.7 | -1.3e-1 | -2.0 | -1.9 | -1.4 | 4.1e-1 | -4.3 | 1.3 |
| D187 | 8.6e-1 | 6.2e-1 | 1.6 | 7.6e-1 | -2.3 | -8.4e-1 | -1.6 | 2.9 | 1.7 | 5.0e-1 |
| R188 | -6.8e-1 | 5.2e-1 | 1.9 | -2.0e-1 | -2.6 | -3.1 | -2.1e-1 | -1.4e-1 | -7.9e-1 | 4.1e-1 |
| Q189 | -7.9e-1 | -3.2e-1 | 7.4e-1 | 8.8e-1 | -8.7e-1 | 2.6e-1 | -2.1e-1 | 4.9e-1 | 3.6e-1 | 6.9e-2 |
| T190 | 9.3e-1 | 6.4e-1 | 2.0 | 2.2 | 4.1e-1 | 1.6 | n/a | 2.6e-1 | 1.6 | 8.2e-1 |
| Q192 | 9.0e-1 | -1.6 | 4.5 | 1.1 | 7.7e-1 | 6.7e-1 | -1.6 | 1.4 | 9.0e-1 | 3.2 |
| **P132** | -1.1e-1 | 1.2 | 3.0e-1 | 9.0e-1 | n/a | 5.5e-1 | 1.2 | 1.7 | 2.2e-1 | -6.0e-1 |

Each residue at the nirmatrelvir binding site or the Omicron variant mutation site (P132, in bold font) is evaluated for 19 potential mutations, whereby the BA change (10 × kcal/mol) relative to the WT is calculated as ΔBA=BA(mut)-BA(WT). Note, BA is related to p$K_i$ as 1.363*p$K_i$. The entries for the WT are shown as n/a.

Table S5: Experimental IC50 and $K_i$ values of nirmatrelvir against mutants of SARS-CoV-2 Mpro and labels for potential drug resistance

| Mutation | IC50(nM) | pIC50 | $K_i$(nM) | p$K_i$ | Label | Mutation | IC50(nM) | pIC50 | $K_i$(nM) | p$K_i$ | Label |
|---|---|---|---|---|---|---|---|---|---|---|---|
| WT | 26.03 | 7.585 | 1.88 | 8.726 | n/a | H172L | 3380 | 5.471 | 3135 | 5.504 | 1 |
| N142Y | 14.9 | 7.827 | | | 0 | H172M | 699 | 6.156 | 290.6 | 6.537 | 1 |
| N142T | 18.73 | 7.727 | | | 0 | H172A | 374.7 | 6.426 | 213.8 | 6.670 | 1 |
| N142K | 13.93 | 7.856 | | | 0 | H172I | 10000 | 5.000 | 10000 | 5.000 | 1 |
| N142D | 24.3 | 7.614 | | | 0 | H172N | 1827 | 5.738 | 1613 | 5.792 | 1 |
| N142L | 15.29 | 7.816 | | | 0 | H172S | 5650 | 5.248 | 2204 | 5.657 | 1 |
| N142S | 25.97 | 7.586 | | | 0 | H172Q | 152.1 | 6.818 | 70.54 | 7.152 | 1 |
| N142I | 17.11 | 7.767 | | | 0 | H172K | 1030 | 5.987 | | | 1 |
| N142H | 19.65 | 7.707 | | | 0 | H172R | 10000 | 5.000 | | | 1 |
| N142M | 19.01 | 7.721 | | | 0 | H172G | 810.2 | 6.091 | | | 1 |
| S144D | 8532 | 5.069 | | | 1 | H172C | 3056 | 5.515 | | | 1 |
| S144K | 10000 | 5.000 | 10000 | 5.000 | 1 | H172V | 10000 | 5.000 | | | 1 |
| S144R | 6134 | 5.212 | 2190 | 5.660 | 1 | H172F | 212.2 | 6.673 | 46.6 | 7.332 | 1 |
| S144M | 175 | 6.757 | 79.26 | 7.101 | 1 | H172T | 10000 | 5.000 | 12672 | 4.897 | 1 |
| S144F | 133.3 | 6.875 | 47.23 | 7.326 | 1 | H172Y | 279.3 | 6.554 | 275.1 | 6.561 | 1 |
| S144G | 96.55 | 7.015 | 27.98 | 7.553 | 1 | H172D | 266.1 | 6.575 | 170.6 | 6.768 | 1 |
| S144A | 171.1 | 6.767 | 36.43 | 7.439 | 1 | H172E | 10000 | 5.000 | | | 1 |
| S144Y | 61.49 | 7.211 | 34.09 | 7.467 | 1 (0) | Q189F | 34.02 | 7.468 | | | 0 |
| S144L | 5364 | 5.271 | 3952 | 5.403 | 1 | Q189R | 37.82 | 7.422 | | | 0 |
| S144T | 353.7 | 6.451 | 207.1 | 6.684 | 1 | Q189H | 32.71 | 7.485 | | | 0 |
| S144P | 10000 | 5.000 | 10000 | 5.000 | 1 | Q189L | 39.25 | 7.406 | | | 0 |
| S144W | 289.6 | 6.538 | 143.8 | 6.842 | 1 | Q189P | 14.08 | 7.851 | | | 0 |
| S144E | 423.4 | 6.373 | 153.2 | 6.815 | 1 | Q189S | 25.34 | 7.596 | | | 0 |
| S144V | 1442 | 5.841 | 858.9 | 6.066 | 1 | Q189E | 49.71 | 7.304 | 4.51 | 8.346 | 0 |
| S144H | 650.5 | 6.187 | 402.2 | 6.396 | 1 | Q189K | 39.31 | 7.405 | 14.6 | 7.836 | 0 |
| S144Q | 831.2 | 6.080 | 576.8 | 6.239 | 1 | Q192F | 92.68 | 7.033 | 85.5 | 7.068 | 1 |
| H164N | 32.85 | 7.483 | 3.58 | 8.446 | 0 | Q192K | 219.1 | 6.659 | 88.9 | 7.051 | 1 |
| M165T | 94.68 | 7.024 | 52.68 | 7.278 | 1 | Q192L | 121.9 | 6.914 | 70.99 | 7.149 | 1 |
| M165Y | 10462 | 4.980 | 7216 | 5.142 | 1 | Q192S | 217.3 | 6.663 | 75.56 | 7.122 | 1 |
| M165F | 1336 | 5.874 | | | 1 | Q192A | 140.7 | 6.852 | 58.1 | 7.236 | 1 |
| M165H | 10000 | 5.000 | | | 1 | Q192I | 109.9 | 6.959 | 43.53 | 7.361 | 1 |
| M165P | 10000 | 5.000 | | | 1 | Q192P | 135.1 | 6.869 | 76.19 | 7.118 | 1 |
| M165R | 10000 | 5.000 | | | 1 | Q192G | 319.1 | 6.496 | 106.3 | 6.973 | 1 |
| M165W | 10000 | 5.000 | | | 1 | Q192E | 193.1 | 6.714 | 114.4 | 6.942 | 1 |
| M165K | 10000 | 5.000 | | | 1 | Q192H | 169.4 | 6.771 | 80.69 | 7.093 | 1 |
| M165L | 22.62 | 7.646 | 1.04 | 8.983 | 0 | Q192T | 102.6 | 6.989 | 45.69 | 7.340 | 1 |
| M165I | 27.38 | 7.563 | 2.02 | 8.695 | 0 | Q192V | 95.58 | 7.020 | 30.87 | 7.510 | 1 |
| M165V | 23.96 | 7.621 | | | 0 | Q192W | 65.94 | 7.181 | 43.65 | 7.360 | 1 |
| M165A | 23.28 | 7.633 | | | 0 | Q192C | 96.82 | 7.014 | 54.12 | 7.267 | 1 |
| M165G | 243.5 | 6.614 | | | 0 | Q192D | 271.5 | 6.566 | | | 1 |
| M165C | 24.84 | 7.605 | | | 0 | Q192Y | 10000 | 5.000 | | | 1 |
| M165D | 147.6 | 6.831 | | | 0 | Q192N | 73.69 | 7.133 | | | 0 |
| E166I | 10000 | 5.000 | | | 1 | Q192R | 229.6 | 6.639 | | | 0 |
| E166G | 92.15 | 7.036 | 30.89 | 7.510 | 1 | M49L | 18.5 | 7.733 | 1.57 | 8.804 | 0 |
| E166V | 10000 | 5.000 | 10384 | 4.984 | 1 | M49T | 15.76 | 7.802 | 2 | 8.699 | 0 |
| E166A | 152 | 6.818 | 89.29 | 7.049 | 1 | M49V | 23.48 | 7.629 | | | 0 |
| E166Y | 3711 | 5.431 | | | 1 | M49I | 26.54 | 7.576 | | | 0 |
| E166H | 9598 | 5.018 | | | 1 | | | | | | |
| E166K | 1994 | 5.700 | | | 1 | | | | | | |
| E166Q | 27.87 | 7.555 | 8.37 | 8.077 | 0 | | | | | | |
| E166L | 214.2 | 6.669 | | | 0 | | | | | | |

Experimental data taken from Hu et al.,[S1] with double mutants excluded. p$K_i$ =-$\log_{10} K_i$ and pIC50 = -$\log_{10}$IC50. A mutation is labeled as potentially drug resistance if p$K_i$(mut)−p$K_i$(WT) $<$ -1 or pIC50(mut)−pIC50(WT) $<$ -1 (if $K_i$ is unavailable).

Table S6: Potential drug-resistance mutations predicted by PARAmount

| Mutation | $\Delta$BA | Status | Mutation | $\Delta$BA | Status |
|---|---|---|---|---|---|
| M49L | -0.16 | FP | H164Y | -0.13 | TBT |
| M49T | -0.16 | FP | L167S | -0.10 | TBT |
| **F140L** | -0.14 | TP | **H172Y** | -0.43 | TP |
| N142D | -0.13 | FP | R188S | -0.31 | TBT |
| N142T | -0.15 | FP | T190A | -0.16 | TBT |
| G143S | -0.13 | TBT | | | |

Predicted $\Delta$BAs are given in kcal/mol. Mutations confirmed by experiments[S1,S26,S27] are highlighted. The status column lists three values: true positive, false positive, and to be tested (TBT) for predictions awaiting experimental verification.

# Supplementary Figures

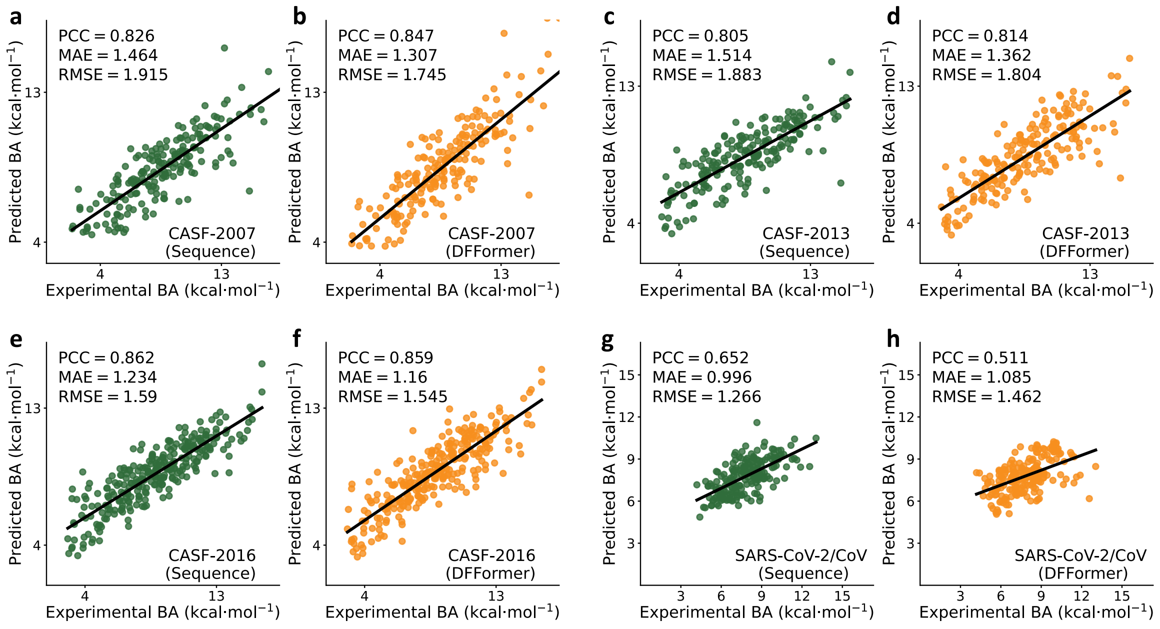


Figure S1: Performances of DFFormer and Seq-trees in predicting protein-ligand BAs from the CASF and SARS-CoV/CoV-2 Mpro datasets. Comparison between the predicted and experimental BAs using the Seq-ML model (**a, c, e, g**) and the DFFormer model (**b, d, f, h**). Note, for the SARS-CoV/CoV-2 Mpro dataset, the 5-fold CV is shown.

# Supplementary Mathematical Methods

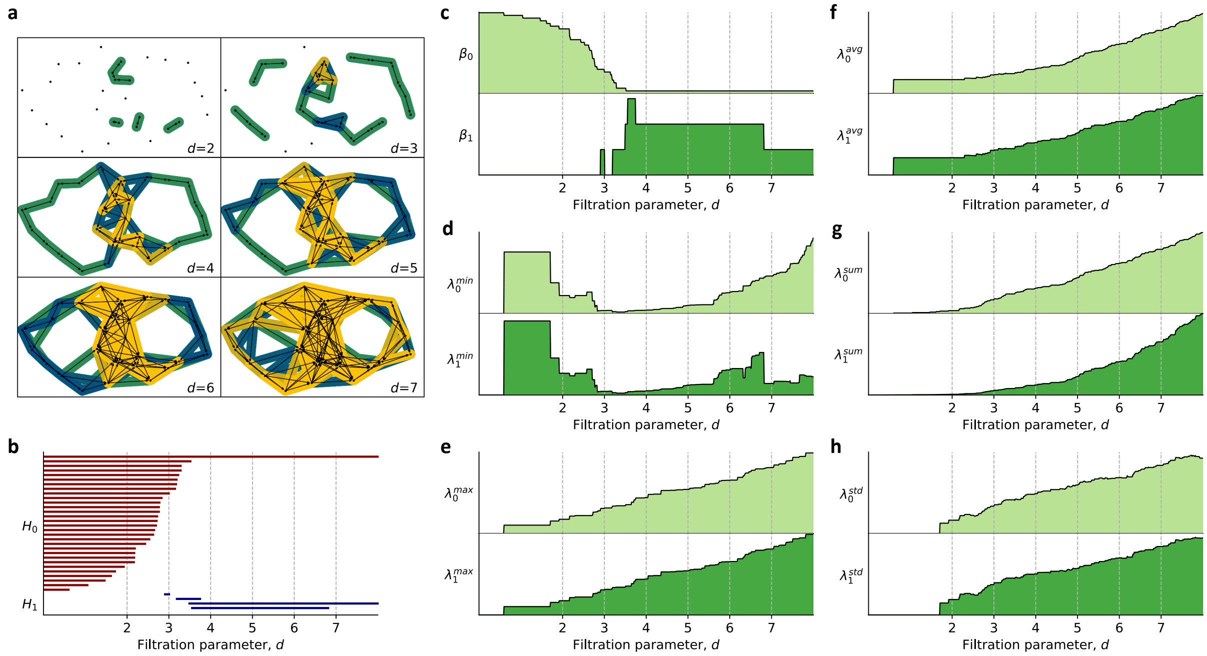


Figure S2: Analysis of persistent directed flag Laplacian versus persistent directed flag homology for the point cloud shown in main text Figure 5**a**. **a**, How varying the filtration parameter alters the connectivity of the point cloud, leading to a sequence of directed flag complexes that represent different topological structures. **b**, The barcodes for persistent directed flag homology groups $H_0$ and $H_1$ at the 0th and 1st dimensions, respectively, highlighting their changes due to the filtration (or scale) parameter $d$. **c**, Visualization of the variations in the topological invariants at the 0th ($\beta_0$) and 1st ($\beta_1$) dimensions of the persistent directed flag complex as a function of $d$. **d**, Representation of the nonzero minimum non-harmonic spectra of the persistent directed flag Laplacian at the 0th and 1st dimensions ($\lambda_0^{min}$ and $\lambda_1^{min}$), emphasizing their dependence on $d$. **e**, Representation of the maximum non-harmonic spectra of the persistent directed flag Laplacian at the 0th and 1st dimensions ($\lambda_0^{max}$ and $\lambda_1^{max}$), emphasizing their dependence on $d$. **f**, The average values of nonzero spectra for the persistent directed flag Laplacian in both the 0th and 1st dimensions ($\lambda_0^{avg}$ and $\lambda_1^{avg}$). **g**, The standard deviation of nonzero spectra for the persistent directed flag Laplacian in the 0th and 1st dimensions ($\lambda_0^{std}$ and $\lambda_1^{std}$). **h**, The sum of nonzero spectra values for the persistent directed flag Laplacian in the 0th and 1st dimensions ($\lambda_0^{sum}$ and $\lambda_1^{sum}$).

Fig. S2 illustrates the persistent characteristics obtained from the non-harmonic spectra of a persistent directed flag Laplacian in both the 0th and 1st dimensions. By incrementally modifying $d$, a series of hierarchical data representations can be obtained (Fig. S2**a**). Panel **e** shows the progression of zero eigenvalue multiplicities in the corresponding Laplacian matrix as the filtration parameter ($d$) evolves, while Panel **f** and **g** show the changes in the nonzero minimum and maximum positive eigenvalue as $d$ varies. Panel **d** shows the persistent barcodes for homology groups $H_0$ and $H_1$ in the 0th and 1st dimensions, respectively. The topological invariants,

specifically the Betti numbers, correspond to the frequency of the zero eigenvalue in the directed flag Laplacian for a specific $d$. It is important to note that these persistent attributes change with varying $d$, thereby capturing both topological and geometric data in a multiscale fashion.

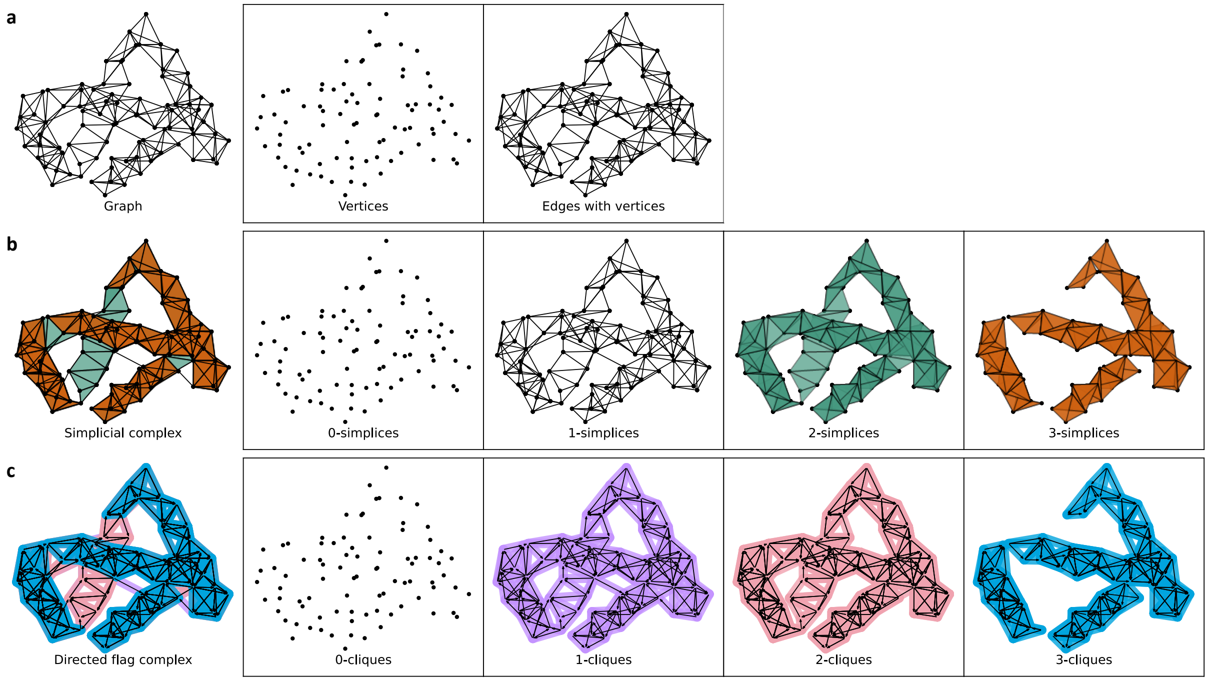


Figure S3: Illustration of different representations of a protein based on the $C_\alpha$ atoms (PDBID: IMYL). **a** A graph representation of the structure. **b** The simplicial complex representation of the structure, including a list of 0-simplices, 1-simplices, 2-simplices, and 3-simplices in the complex. **c** A directed flag complex representation of the structure, along with a list of 0, 1, 2, and 3-clique within the directed flag complex.

Figure S3 shows a variety of topological representations of a protein based on $C_\alpha$ atoms (PDBID: IMYL) and a pairwise cutoff distance of 5 Å. In Panel **a**, the traditional graph representation of the protein structure is displayed. Building on this graph representation, the 0-simplices in the simplicial complex are equivalent to the vertices in the graph, and the 1-simplices correspond to edges connecting these vertices, as demonstrated in the second and third columns of Panels **a** and **b**. Additionally, higher-dimensional simplices within the simplicial complex reveal more complex aspects of the structure. For example, 3-simplices can approximate the structure of alpha helices. With the directional attributes, directed flag complexes offer a more comprehensive representation than simplicial complexes. Directed flag complexes incorporate cliques of various dimensions, thus capturing multilevel structural information, as depicted in Panel **c**.

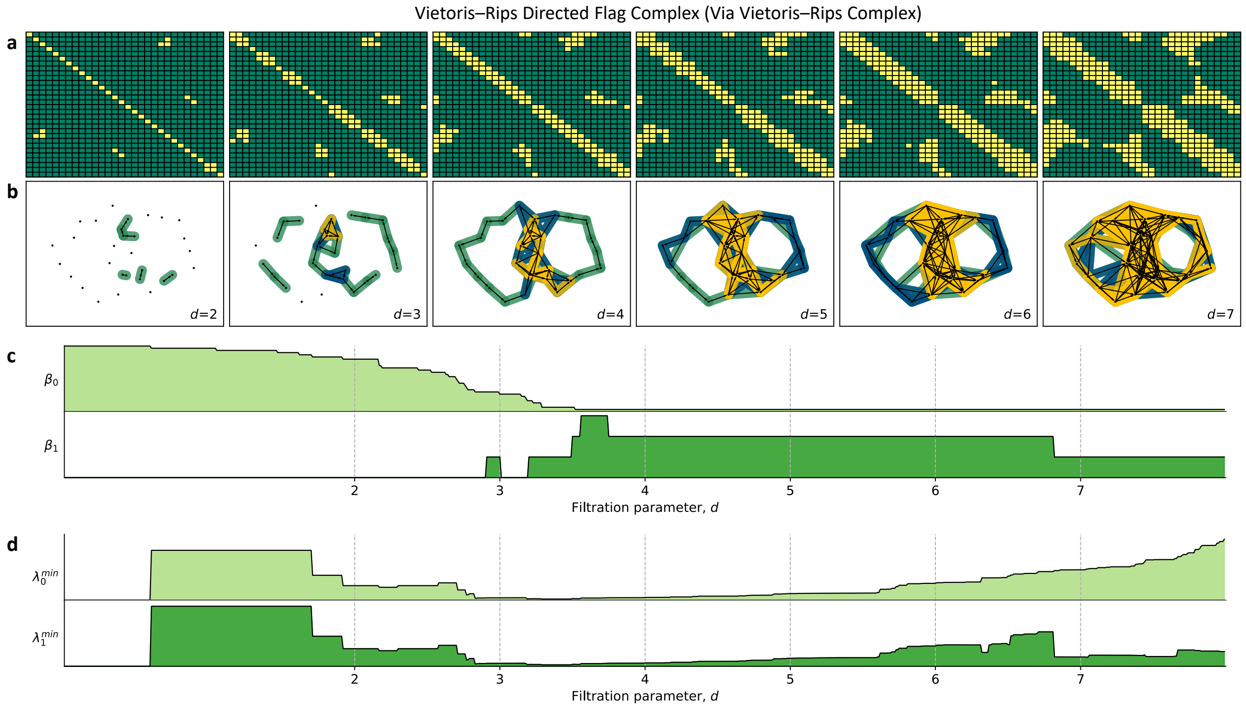


Figure S4: Illustration of Vietoris-Rips directed flag complex across various scales for the point cloud shown in the main text Figure 5**a**. **a** The adjacency matrices of the point cloud at different scales, are characterized by the filtration parameter $d$. Yellow entries represent connected points with a distance below the chosen cutoff, whereas green entries mark points that are not connected. **b** The Vietoris-Rips directed flag complexes constructed at multiple scales are displayed with $d$ = 2, 3, 4, 5, 6, or 7. **c** The persistent Betti numbers, labeled as $\beta_i$ for $i = 0$ and $i = 1$. The specific scales at which these Betti numbers occur are indicated by vertical dashed lines. **d** The minimum non-harmonic spectra (non-zero) of the persistent directed flag Laplacian in both the 0th and 1st dimensions ($\lambda_0^{min}$ and $\lambda_1^{min}$), emphasizing how these values vary with the scale parameter $d$.

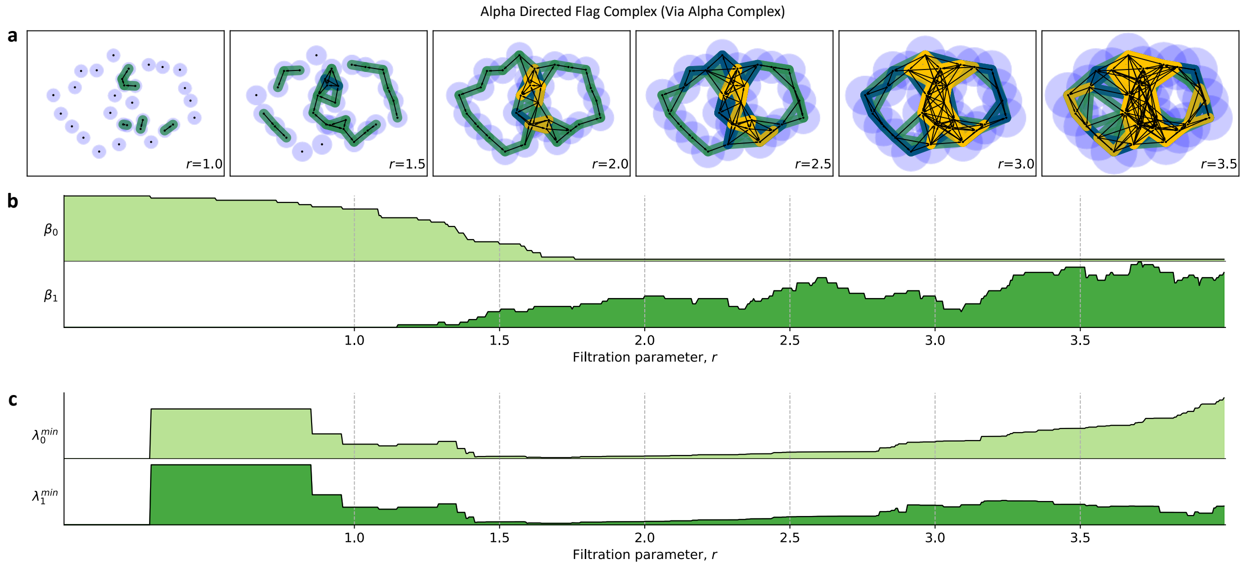


Figure S5: Illustration of building an alpha directed flag complex from the alpha complex with varying scale parameters for the point cloud shown in Figure 5**a**. **a** The constructed alpha directed flag complexes at a given filtration parameter, i.e., $r = 1.0$, $r = 1.5$, $d = 2.0$, $d = 2.5$, $d = 3.0$, and $d = 3.5$. **b** The persistent Betti numbers of alpha directed flag complexes, $\beta_i, i = 0, 1$. The vertical dash lines indicate the Betti numbers at a given filtration parameter. **c** Representation of nonzero minimum non-harmonic spectra of the persistent directed flag Laplacian at the 0th and 1st dimensions ($\lambda_0^{min}$ and $\lambda_1^{min}$) for alpha directed flag complex, highlighting their dependence on the filtration parameter.

## Directed flag topological sequence embedding

**Directed flag complex.** A directed flag complex is a conceptual extension of graphs, directed graphs, and simplicial complexes, serving as a combinatorial and topological structure derived from a directed graph (digraph). This framework generalizes the simplicial complex by incorporating directionality into the underlying graph. In Figure 5**b**, examples of the building blocks of the directed flag complex for various dimensions, such as 0-cliques, 1-cliques, 2-cliques, and 3-cliques, are presented. These structures embed directional information into the simplicial complex, contrasting with the $0$-simplex (a single node), $1$-simplex (a line segment), $2$-simplex (a triangle), and $3$-simplex (a tetrahedron) illustrated in Figure 5**c**.

In mathematical terms, given a directed graph $G = (V, E)$, where $V$ is the set of vertices and $E \subseteq V \times V$ is the set of directed edges, the directed flag complex (or directed clique complex) of a directed graph $G$ is a simplicial complex where the vertices of the directed flag complex correspond to the vertices of $G$, and a $k$-clique (also refer to directed $k$-simplex) in the directed flag complex corresponds to a directed $(k+1)$-clique in $G$. That is, a subset of $k+1$ vertices $\{v_0, v_1, \ldots, v_k\} \subset V$ such that $(v_i, v_j) \in E$ for all $i < j$. The clique here means the complete subgraph here.

**Vietoris-Rips directed flag complex and alpha directed flag complex.** The Vietoris-Rips (VR) complex and the alpha complex are highly regarded topological models for analyzing sets of data points. In cases where $\mathcal{K}$ is a VR complex or an alpha complex, the points that comprise a simplex in $\mathcal{K}$ inherently encapsulate geometric information, including both the size and orientation of the set of points. Drawing inspiration from the VR complex and the alpha complex, we introduce the Vietoris-Rips (VR) directed flag complex and the alpha directed flag complex, aimed at capturing this geometric information. To describe the geometry of simplices, a weight function $w : \mathcal{K} \to \mathbb{R}$ and a graded orientation function $\varrho_n : \mathcal{K}_n \to S_{n+1}$ for $n \geq 1$ are employed. In this context, $S_n$ represents the permutation group with $n$ elements. The VR/alpha

directed flag complex is formulated as follows:

$$\mathcal{DF}_\eta := \{S \times \varrho_*(S) \mid w(S) \leq \eta, S \in \mathcal{K}\}.$$

The VR/alpha directed flag complex can be viewed as an extension of the conventional VR/alpha complex. It reduces to the standard VR/alpha complex when the functions $w : \mathcal{K} \to \mathbb{R}$ and $\varrho_n : \mathcal{K}_n \to S_{n+1}$ are considered constant.

In this study, unless explicitly stated otherwise, all analyses are based on the Vietoris-Rips (VR) directed flag complex. Illustrative examples of the VR directed flag complex and the alpha directed flag complex can be seen in Figures S4 and S5.

**Topological deep learning** Topological deep learning (TDL) was introduced in 2017 for topology-based deep convolutional and multi-task neural networks for biomolecular property predictions.[S28] The early development was based on persistent homology,[S29,S30] a vital tool in topological data analysis.[S31,S32] TDL was the top winner in DR3 Grand Challenges, a worldwide annual competition series in computer-aided drug design,[S33,S34] demonstrating the power of algebraic topology in biomolecular modeling and prediction. Over the years, TDL has become an emerging paradigm in data science.[S35] However, persistent homology has many limitations.[S36] Some of these limitations were addressed by persistent Laplacians,[S37,S38] including persistent directed flag Laplacians.[S39]

**Directed flag Laplacians and spectrum analysis.** The combinatorial Laplacian is a key instrument in discrete geometry and algebraic topology, providing insights into the structure of various topological systems.[S36] These include simplicial complexes,[S37] directed flag complexes,[S39] cellular sheaves,[S40] path complexes,[S41,S42] hypergraphs,[S43] and hyperdigraphs.[S44] Analogous to how the graph Laplacian is utilized for examining graph properties (with graphs being equivalent to 1-simplices), the combinatorial Laplacian is employed for exploring attributes of simplicial and directed flag complexes. The eigenvalues of the graph Laplacian reveal connectivity aspects of

the graph. For instance, the second-smallest eigenvalue, known as the Fiedler vector, indicates the graph's algebraic connectivity. Similarly, the smallest positive eigenvalue, referred to as the spectral gap, has a significant relation to the Cheeger constant. The entirety of these eigenvalues forms the spectrum of the Laplacian operator.

The Laplacian matrix of a graph is defined as $\mathcal{L} = D - A$, where $D$ is the degree matrix, and $A$ is the adjacency matrix. In the context where the graph is considered as a one-dimensional (1D) simplicial complex, and taking $B_1$ as the matrix that represents the 1D boundary operator, we find that the graph Laplacian matrix can be accurately formulated as $\mathcal{L} = B_1 B_1^T$. This observation paves the way for extending the Laplacian operator to higher dimensions through the use of the boundary operator, culminating in the Laplacian operator for simplicial complexes. Suppose $K$ represents a simplicial complex, and $B_k$ signifies the matrix of its $k$-dimensional boundary operator. The Laplacian matrix in this context is given by:

$$\mathcal{L}_k = B_{k+1}B_{k+1}^T + B_k^T B_k. \tag{1}$$

In this equation, $B_k^T$ is the transpose of $B_k$. The expression $B_k^T B_k$ reflects the connectivity that arises at the juncture of $k$-simplices at $(k-1)$-simplices. In contrast, $B_{k+1}B_{k+1}^T$ represents the interactions that occur due to the incorporation of $k$-simplices into $(k+1)$-simplices.

Recall that the topological characteristics of simplicial complexes or directed flag complexes are obtained from their chain complexes. The Laplacian operator can be defined from the perspective of chain complexes. Consider $C_*$ as a chain complex with real coefficients, equipped with the differential $\partial_k : C_k \to C_{k-1}$. We assume that for each $k$, $C_k$ is endowed with an inner product structure. As a result, the boundary operator $\partial_k$ is paired with its adjoint operator $\partial_k^*$. The *combinatorial Laplacian* $\Delta_k : C_k \to C_k$ is then defined as

$$\Delta_k = \partial_{k+1} \circ \partial_{k+1}^* + \partial_k^* \circ \partial_k. \tag{2}$$

In particular, $\Delta_0$ is given by $\partial_1 \circ \partial_1^*$. For each $k$, after selecting a standard orthonormal basis

for $C_k$, the corresponding representation matrix $L_k$ of the Laplacian operator $\Delta_k$, relative to this basis, is expressed as form in Equation 1, where $B_k$ represents the matrix corresponding to the boundary operator $\partial_k$, as determined by multiplication to the left.[S45]

This combinatorial Laplacian expands upon the graph Laplacian, which primarily addresses properties of graphs, conceptualized as 1-simplicial complexes. In contrast, the combinatorial Laplacian extends the analysis to higher dimensions. Its eigenvalues and eigenvectors reveal significant geometric and topological details about the simplicial or directed flag complex. Given that the Laplacian matrix is positive semidefinite, all its eigenvalues are nonnegative. The zero eigenvalues, forming the harmonic spectrum, are particularly informative of the topological structure. Meanwhile, the non-zero eigenvalues, or the non-harmonic spectrum, convey the geometric aspects of the system. In the case of $\mathcal{L}_k$, the frequency of zero eigenvalues (indicating the number of occurrences of 0 as an eigenvalue) corresponds to the count of independent components and also to the topological invariants ($\beta_k$) in the $k$-dimensional space.[S46] For example, the zero multiplicity for $\mathcal{L}_0$ (i.e., $\beta_0$) represents the count of connected components in the graph (1-simplicial complex), for $\mathcal{L}_1$ (i.e., $\beta_1$) it denotes the number of cycles, and for $\mathcal{L}_2$, it signifies the number of cavities. The highest eigenvalue $\lambda_k^{max}$ of $\mathcal{L}_k$ is bounded by the maximal count $d_k$ of $k+1$-simplices sharing a common $k$-simplex (akin to the maximum degree of the graph for $\mathcal{L}_0$), so $0 \leq \lambda_k^{max} \leq 2d_k$. The smallest non-zero eigenvalue of $\mathcal{L}_k$, known as the spectral gap and denoted by $\lambda_k^{min}$, reflects the geometric structure of the system. This work utilizes various measures like the multiplicity of zero, the average, the standard deviation, the minimum, the maximum, and the sum of the positive eigenvalues of $\mathcal{L}_0$ for embedding given topological Laplacians.

**Persistent directed flag Laplacians.** Persistent Laplacians, also known as multiscale/persistent topological Laplacians, emerged from a collection of studies conducted on differential manifold settings[S47] and discrete point cloud scenarios.[S37] Central to the concept of persistent Laplacians,[S37,S44,S48] as well as in persistent homology,[S29,S30] is the process of filtration, which facilitates multiscale representation. This filtration, characterized by the scale parameter denoted

as $d$, is tailored according to the specific data structure under examination. For example, in the context of point cloud data (as shown in Figure 5**a**), this parameter typically represents the radius (or diameter) of a sphere. By incrementally modifying $d$, a series of hierarchical data representations can be obtained, as depicted in Figure S2**a**. Importantly, these representations extend beyond simplicial complexes to include structures such as directed flag complexes.[S39] For example, in the context of a distance matrix in which matrix elements denote distances between vertices, a filtration operation can be implemented. Here, a cutoff value is designated as the scale parameter, and if the distance between two vertices is less than this cutoff, an edge is established. As this cutoff value increases, a sequence of nested graphs is formed, where each graph, corresponding to a lower cutoff value, forms a subset of the graphs generated at higher cutoffs.

Similarly, nested simplicial complexes can be constructed using different complex formulations such as the Vietoris-Rips complex, the Čech complex, and the alpha complex. In this study, the focus is on the Vietoris-Rips complex. Mathematically, these nested simplicial complexes are represented as follows:

$$\emptyset \subseteq K_{d_0} \subseteq K_{d_1} \subseteq \cdots \subseteq K_{d_n} = K \tag{3}$$

Here, it holds that for any two values $d_i < d_j$, the complex $K_{d_i}$ is a subset of $K_{d_j}$. This concept is also applicable to directed flag complexes, specifically through the Vietoris-Rips directed flag complex framework, where nested directed flag complexes are formed by defining directed edges in a particular manner.[S39] To illustrate the impact of varying the filtration parameters, Figure S2**a** demonstrates changes in point cloud connectivity from Figure 5**a**, resulting in a progression of directed flag complexes. The methodology for constructing the Vietoris-Rips directed flag complex is detailed in Figure S4. Furthermore, this work introduces the concept of the alpha directed flag complex, inspired by the alpha complex, as depicted in Figure S5.

During the progression of a filtration process, a series of chain complexes naturally emerges. Upon each filtration step, denoted $d_i$ (with $i$ serving as the step index), a distinct chain complex $C(K_{d_i}; G)$ is formed. In mathematical terms, a chain complex associated with a specific

filtration step consists of a sequence of Abelian groups (or modules) connected by boundary homomorphisms, which can be represented as follows:

$$\cdots \to C_{k+1}(K_{d_i};G) \xrightarrow{\partial_{k+1}^{d_i}} C_k(K_{d_i};G) \xrightarrow{\partial_k^{d_i}} C_{k-1}(K_{d_i};G) \to \cdots \tag{4}$$

In this sequence, $C_k(K_{d_i};G)$ denotes the chain group in the $k$-dimensional space at the specific filtration step $d_i$.

To provide a broader understanding, we will now present the Laplacian in a more comprehensive mathematical framework. Consider two real numbers, $a$ and $b$, with $a \leq b$. Let chain complex $C_*^a$ be a subset of $C_*^b$. The chain complexes in question could be derived from a variety of sources, such as filtration of simplicial complexes, directed flag complexes, or hyperdigraphs, to name a few. Furthermore, it is important to note that both $C_*^a$ and $C_*^b$ possess compatible inner product structures. Let $C_{k+1}^{a,b}$ be a set containing elements $x$ in $C_{k+1}^b$ such that the boundary operator $\partial_{k+1}^b$ applied to $x$ produces an element in $C_k^a$, formally expressed as $C_{k+1}^{a,b} = \{x \in C_{k+1}^b | \partial_{k+1}^b x \in C_k^a\}$.

The persistent boundary operator, denoted as $\partial_{k+1}^{a,b}$ and mapping from $C_{k+1}^{a,b}$ to $C_k^a$, is defined through the action $\partial_{k+1}^{a,b} x = \partial_{k+1}^b x$ for any $x$ residing in $C_{k+1}^{a,b}$. This operator plays a key role in understanding persistent structures within the framework of chain complexes. The *$k$-th persistent Laplacian* is defined as

$$\Delta_k^{a,b} = \partial_{k+1}^{a,b} \circ (\partial_{k+1}^{a,b})^* + (\partial_k^a)^* \circ \partial_k^a. \tag{5}$$

It is important to recognize that the harmonic part of $\Delta_k^{a,b}$, denoted $\ker \Delta_k^{a,b}$, has a natural isomorphism to the $(a,b)$-persistent homology, expressed as $H_k^{a,b} = \mathrm{im}(H_k(C_*^a) \to H_k(C_*^b))$.[S49] Essentially, the persistent Laplace harmonic component contains information related to persistent homology. To extract valuable information from each chain complex, spectrum analysis is a viable approach. This involves constructing Laplacian matrices for each $\partial_k$ and $\partial_{k+1}$ and analyzing their spectra (eigenvalues and eigenvectors), which can reveal in-depth information about the topological and geometric attributes inherent in the data at a specific filtration scale. The spectral data often offer a concise and informative representation of the data, facilitating effective

comparison and analysis across various scales. The persistent attributes used in this work are shown in Figure S2. This approach underscores the multifaceted nature of persistent topological Laplacians in capturing and representing complex topological and geometric structures.

**Element-specific embedding.** In this study, the directed flag topological embedding method is used to encode protein-ligand complexes, with the aim of improving the prediction accuracy by better representing the molecular interactions between proteins and ligands. The element-specific topological embedding approach[S28,S50] is utilized to represent these interactions.

When analyzing ligands, attention is focused on heavy elements like carbon (C), nitrogen (N), oxygen (O), sulfur (S), phosphorus (P), fluoride (F), chloride (Cl), bromide (Br), and iodine (I). In the context of proteins, the analysis is limited to carbon (C), nitrogen (N), oxygen (O), and sulfur (S). A series of element combinations, ordered in a specific sequence, are then employed to represent the interactions between the protein and the ligand. For proteins, the combinations are denoted as $\mathcal{E}_{\rm protein}$={{C}, {N}, {O}, {S}, {C, N}, {C, O}, {C, S}, {N, O}, {N, S}, {O, S}, {C, N, O, S}}. Similarly, the ligand combinations are represented as $\mathcal{E}_{\rm ligand}$={{C}, {N}, {O}, {S}, {C, N}, {C, O}, {C, S}, {N, O}, {N, S}, {O,S}, {N, P}, {F, Cl, Br, I}, {C, O, N, S, F, P, Cl, Br, I}}. In the Element-specific embedding framework, protein-ligand interactions are delineated through the topological links between two distinct sets of atoms: one set from the protein and the other from the ligand. For instance, a configuration like $K_{\{\rm C,N\},\{\rm S\}}$ signifies a directed flag complex where the carbon (C) and nitrogen (N) atoms are part of the protein, while the sulfur (S) atom is part of the ligand. This Element-specific embedding methodology provides a detailed depiction of interactions, focusing on their spatial arrangements and relationships. It can be characterized by distance matrix $D$ as follows,

$$D(i,j) = \begin{cases} \|\mathbf{r}_i - \mathbf{r}_j\|, & \text{if } \mathbf{r_i} \in \mathcal{E}_{\rm protein}, \mathbf{r_j} \in \mathcal{E}_{\rm ligand} \text{ or } \mathbf{r_i} \in \mathcal{E}_{\rm ligand}, \mathbf{r_j} \in \mathcal{E}_{\rm protein} \\ \infty, & \text{other} \end{cases} \tag{6}$$

where the $\mathbf{r}_i$ and $\mathbf{r}_j$ are coordinates for the $i$th and $j$th atoms in the set, and $\|\mathbf{r}_i - \mathbf{r}_j\|$ is their

Euclidean distance. In the DFFormer model, the focus is on protein atoms that are situated within a 20 Å radius of ligand atoms. This model prioritizes protein-ligand interactions by designating an infinite distance value for atom pairs that are exclusively within the protein or within the ligand. This approach ensures that the model's attention is directed specifically towards the interactions between protein and ligand atoms. For any given protein-ligand complex under consideration, there are 143 potential combinations (derived from 11 protein sets multiplied by 13 ligand sets). Each combination represents a unique directed flag complex and is subsequently analyzed using the persistent directed flag Laplacian method. This approach allows for an in-depth examination of the various possible interactions within the protein-ligand complex, leveraging the unique properties of each element set to understand the complex interplay between the protein and ligand at a molecular level.

## Topological objects

**Graph.** The graph is a fundamental structure for illustrating relationships among entities, consisting of nodes (vertices) and edges that connect them. Graphs can be enhanced by adding directionality (directed graphs), assigning weights (weighted graphs), or incorporating geometric properties (geometric graphs). Formally, a graph is defined as a pair $(V, E)$, where $V$ is a set of vertices and $E$ is a subset of $V \times V$ representing edges. Tools such as adjacency matrices, degree matrices, and Laplacian matrices describe interactions between vertices and edges, capturing the graph's topological structure. Although graphs are inherently one-dimensional, simplicial complexes can express their higher-dimensional aspects, including structures such as clique complexes, cell complexes, hypergraphs, neighborhood complexes, and Hom complexes.[S51,S52]

**Simplicial complex.** A simplicial complex is a mathematical structure that is used to study the shape and topology of the data. It is composed of simplices, which are generalizations of points (0-simplices), line segments (1-simplices), triangles (2-simplices), and their higher-dimensional counterparts. A simplicial complex is formed by combining these simplices in a way that satisfies

certain intersection properties: Any face of a simplex in the complex is also a simplex in the complex, and the intersection of any two simplices is either empty or a shared face. This structure allows for the representation of complex shapes and surfaces by breaking them down into simpler components. Simplicial complexes are widely used in computational topology, particularly in persistent homology, to analyze the multi-scale features of data. They provide a framework for understanding the connectivity, holes, and voids within data, which are crucial for applications in areas such as data analysis, computer graphics, and geometric modeling.

**Directed flag complex** . The directed flag complex is a combinatorial and topological structure associated with a directed graph (digraph). It generalizes the concept of a simplicial complex to account for the directionality in the underlying graph. Directed flag complexes can be particularly useful in areas like computational topology, where they are used to study data that can be represented as a network or a graph, such as social networks, biological networks, and sensor networks. They provide a way to generalize the concept of a graph to capture not just relationships between individual elements but also more complex relationships involving sequences of elements.

# Supplementary Computational Methods and Protocols

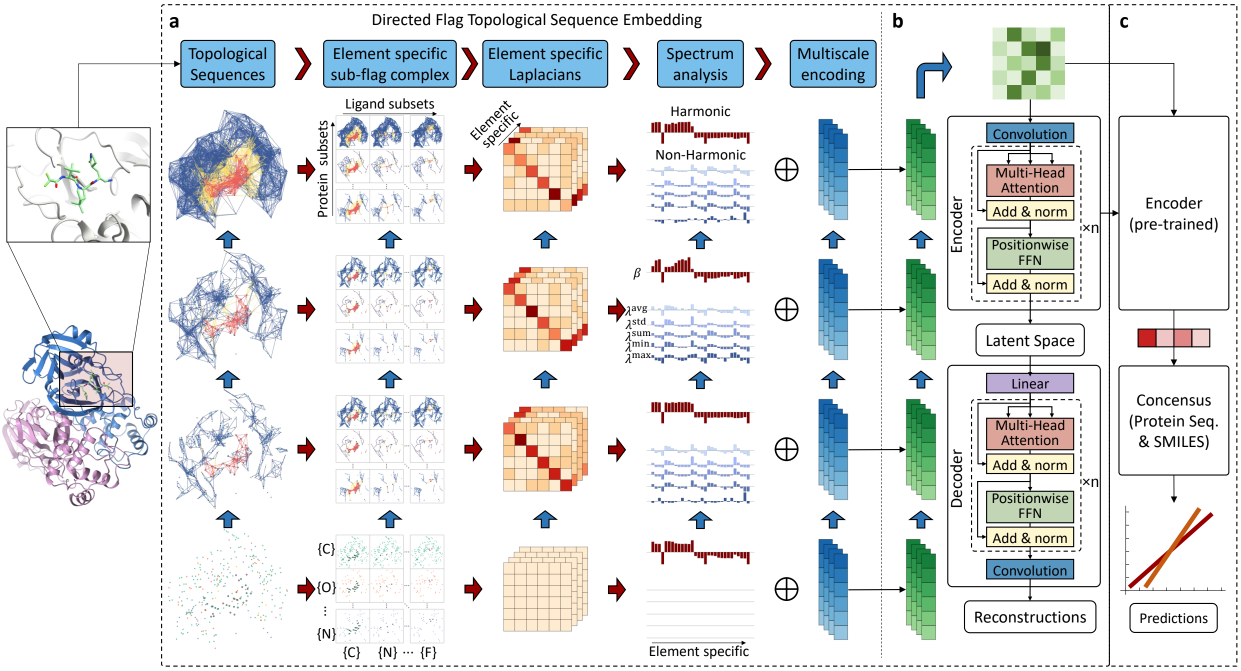


Figure S6: **Schematics of DFFormer.** **a**, A protein-ligand complex is represented by a topological sequence known as a chain complex in algebraic topology. Element-specific sub-complexes are then formed to encode physical interactions at various scales, regulated by a filtration parameter. Element-specific Persistent Topological Directed Flag Laplacians are constructed to extract topological invariants, capturing the shape and stereochemistry of the sub-flag complexes. For these subcomplexes, changes in topological invariants across scales are captured by the harmonic spectrum of the directed flag Laplacians, while their homotopic shape evolution across scales is reflected in the non-harmonic spectrum. Finally, these multiscale topological invariants and homotopic shape (stereochemical) evolutions are compiled into a topological sequence, which serves as input for the transformer. **b**, Self-supervised learning is performed for topological sequences, where the reconstructed sequences are used to compute the loss. **c**, In the supervised fine-tuning stage, the BAs of the protein-ligand complexes are input into the pre-trained encoder. The predictions of DFFormer are combined with those from the sequence-based decision trees to enhance accuracy.

## Architecture of the DFFormer model

**The DFFormer encoder.** DFFormer adopts the architecture of a Masked Autoencoder[S53] (Fig. S1). The Directed Flag Topological Sequence Embedding, once fed into the system, initially passes through a convolution layer. This step is crucial for downsampling the topological embedding and optimizing it for subsequent processing by the encoder module. The convolutional layer is appropriate because the multiscale features from the persistence are related to one another in sequence as the scale parameter varies. Following this convolution layer, the processed embedding advances to multiple encoder layers, each comprising two primary components: a Multi-Head Self-Attention (MHSA) mechanism and a Feed-Forward Neural Network (FFNN). Both components are augmented by normalization layers and incorporate residual connections to enhance the flow of information and learning stability.

The Multi-Head Self-Attention mechanism uses "Scaled Dot-Product Attention". The input of this mechanism consists of queries (Q), keys (K), and values (V), which are all vectors. The attention mechanism is defined as

$$\text{Attention}(Q, K, V) = \text{softmax}\left(\frac{QK^T}{\sqrt{d_k}}\right)V, \tag{7}$$

where $d_k$ is the dimension of the key vectors. This scaling factor $\sqrt{d_k}$ is crucial as it prevents the dot products from growing too large in magnitude, leading to smoother gradients. Specifically, within the framework of DFFormer, each scale's Directed Flag Topological Embedding is adeptly transformed into three distinct vectors: queries (Q), keys (K), and values (V). This transformation is achieved through separate linear transformations, each governed by learnable weights. Subsequently, the attention mechanism is applied to the entire sequence. This process enables each element in the sequence to dynamically attend to every other element, fostering a comprehensive inter-element relationship analysis. Additionally, the Transformer architecture in DFFormer is designed to utilize multiple attention heads, further enhancing its capability to

capture and process complex patterns in the data. Each head learns different aspects of the data:

$$\text{MultiHead}(Q, K, V) = \text{Concat}(\text{head}_1, \text{head}_2, ..., \text{head}_h)W^O, \tag{8}$$

where $h$ is the number of heads, and each head is defined as

$$\text{head}_i = \text{Attention}(QW_i^Q, KW_i^K, VW_i^V) \tag{9}$$

Here, $W_i^Q$, $W_i^K$, $W_i^V$, $W^O$ are parameter matrices.

Beyond the attention mechanism, each encoder layer in the model is equipped with a fully connected feedforward network. This network operates independently and identically on each scale within the layer. This consists of two linear transformations with a GELU (Gaussian Error Linear Unit) activation in between:

$$\text{FFN}(x) = \text{max}(0, xW_1 + b_1)W_2 + b_2 \tag{10}$$

Here, $W_1$, $W_2$, $b_1$, and $b_2$ are learnable parameters. The GELU activation function introduces non-linearity.

Each sublayer (MHSA and FFNN) in the encoder layer is followed by layer normalization and a residual connection. The output of each sub-layer is

$$\text{Output} = \text{LayerNorm}(x + \text{Sublayer}(x)), \tag{11}$$

where $x$ is the input to the sub-layer, Sublayer$(x)$ is the function implemented by the sub-layer itself (either MHSA and FFNN).

**DFFormer decoder.** The DFFormer adopts an asymmetric design, which features a more substantial and complex encoder relative to its decoder. The decoder's primary role in the DFFormer is to reconstruct the original directed flag topological sequence embedding from the

latent representations generated by the encoder. This reconstruction process is pivotal because it compels the decoder to accurately regenerate the directed flag topological sequence, thereby driving the encoder to develop rich and insightful representations of the protein-ligand complex data. Such representations are invaluable for a variety of downstream applications.

Structurally, the layers within the DFFormer Decoder closely mirror those of the DFFormer Encoder. The process begins with the encoder's latent representations being linearly mapped. These mappings are then input into the DFFormer Decoders, which are architecturally similar to the encoder layers in the DFFormer Encoder, albeit with a reduced hidden size. During the pretraining phase, the output from the final decoder layer transforms back into the original directed flag topological sequence, facilitated by a convolution layer. In the fine-tuning stage, the focus shifts to the output derived from the first scale's hidden state, which is utilized for regression tasks, such as binding affinity prediction. Specifically, this output is channeled through a linear layer, culminating in generating the final inference output.

## Binding affinities and related quantities

This study focuses on the prediction of protein-ligand binding affinities (BAs), which is negative binding free energy ($BA = -\Delta G$). Thus, BA is a positive quantity, and a larger BA indicates stronger binding. The conversion from the inhibition constant $K_i$ in unit of M (mol/l) to $BA$ in unit of kcal/mol is quantified by the equation

$$BA = -RT \ln \frac{K_i}{1} \approx -1.3633 \times \log_{10} \frac{K_i}{1} (kcal/mol), \tag{12}$$

where R is the gas constant, T is the temperature (298 K), 1 denotes the standard concentration 1 M or 1 mol/l, and $K_i$ (in unit of M) can be replaced by IC50 if unavailable.

Sometimes, the binding affinity for protein-ligand complex is expressed as

$$pK_i = -\log_{10} \frac{K_i}{1}, \tag{13}$$

which can be converted to BA via $BA = 1.3633 \times pK_i$. A larger $pK_i$ value indicates stronger protein-ligand binding affinity.

In this work, we also consider the change in binding affinity due to mutation, $\Delta BA = BA_{\text{Mutant}} - BA_{\text{WT}}$, where a negative $\Delta BA$ indicates a weakened protein-ligand binding due to the mutation. Similarly, a negative $\Delta pK_i$ also indicates weakened binding affinity.

## Model evaluation metrics

For model evaluations, we used Pearson Correlation Coefficient (PCC) and root-mean-square errors (RMSEs). The PCC is used to describe the relationship between the variables $x$ and $y$. It is defined as

$$\mathrm{PCC} = \frac{\sum (x_i - \bar{x})(y_i - \bar{y})}{\sqrt{\sum (x_i - \bar{x})^2 \sum (y_i - \bar{y})^2}}, \tag{14}$$

where $x_i$ represents the value of $x$ in the $i$th sample, while $\bar{x}$ denotes the average of the $x$ values. Similarly, $y_i$ is the value of $y$ in the $i$th sample, and $\bar{y}$ is the mean of the $y$ values.

The RMSE is defined as

$$\text{RMSE} = \sqrt{\frac{1}{n}\sum_{i=1}^{n} (y_i - \hat{y}_i)^2}, \tag{15}$$

where $y_i$ and $\hat{y}_i$ are the predicted and true values of $i$th sample, respectively.

## Loss function in model training

The Mean Squared Error (MSE) is used as the loss function throughout the pre-training and fine-tuning stages. MSE calculates the average of the squares of the differences between the predicted and actual values, defined as

$$\text{MSE} = \frac{1}{n}\sum_{i=1}^{n}(y_i - \hat{y}_i)^2, \tag{16}$$

where $y_i$ is the actual value for the $i$-th data point, $\hat{y}_i$ is the predicted value for the $i$-th data point, and $n$ is the total number of data points.

## Hyperparameter selection and optimization

In the Seq-tree model, the feature embeddings were extracted from large language models ESM for proteins[S54] and the transformer-CPZ model for small molecules[S55] separately. Following this, the Gradient Boosted Decision Trees (GBDT) algorithm from sklearn library was employed for the prediction of protein-ligand binding affinities. The parameters for the GBDT algorithm were set as follows: 'n_estimators' = 10,000, 'max_depth' = 7, 'min_samples_split' = 2, accompanied by a subsample size of 0.4, and a learning rate of 0.005. All other parameters were in the default settings as specified in the algorithm.[S56] During the prediction phase, the LightGBM algorithm was used due to its faster training and better memory efficiency.[S57] The sequence-based features were trained using this algorithm with the following parameters: 'num_boost_round' set = 10000, 'learning_rate' = 0.01, 'num_leaves' = 125, 'feature_fraction' = 0.9, 'bagging_freq' = 5, 'max_depth' = 7, and 'metric' = 'mse'.

In the DFFormer models, a self-supervised learning method was adopted in the pretraining phase, followed by a supervised learning approach in the fine-tuning stage. Similar to the Masked Autoencoder model[S53] in computer vision, DFFormer employs an asymmetric design in its encoder and decoder. The relevant parameters are given in Table S7.

In the pretraining stage, we tested and selected hyperparameters for effective learning and convergence. We used a batch size of 64 and a maximum of 30,000 training steps, along with an initial learning rate of 0.001 to facilitate gradual and effective weight adjustments. To stabilize the early training phase, we incorporated a warm-up period accounting for 5% of the total training steps, where the learning rate gradually increased from 0 to the initial rate. In the subsequent fine-tuning stage, we employed a supervised learning method to refine the model for specific tasks, focusing on preventing overfitting to the hyperparameters. We decreased the batch size to 32 and modified the initial learning rate to 0.0008. The training steps varied for different tasks, setting a maximum of 10,000 steps for the PDBbind 2020 dataset. For the 5-fold cross-validation task on the SARS-CoV/CoV-2 Mpro dataset, we divided the dataset into five folds, training five separate models. Each model was trained using four out of the five folds, building on the model

Table S7: The parameter settings for DFFormer

| Parameters | Pretraining stage | Fine-tuning stage |
|---|---|---|
| attention_probs_dropout_prob | 0.1 | 0.1 |
| decoder_hidden_size | 768 | / |
| decoder_intermediate_size | 3072 | / |
| decoder_num_attention_heads | 12 | / |
| decoder_num_hidden_layers | 8 | / |
| hidden_act | gelu | gelu |
| hidden_dropout_prob | 0.1 | 0.1 |
| hidden_size | 1024 | 1024 |
| image_size(large) | (100, 143) | (100, 143) |
| image_size(small) | (50, 143) | (50, 143) |
| initializer_range | 0.02 | 0.02 |
| intermediate_size | 4096 | 4096 |
| num_attention_heads | 4096 | 4096 |
| num_channels | 6 | 6 |
| num_hidden_layers | 12 | 12 |
| patch_size | (1, 143) | (1, 143) |

already fine-tuned with PDBbind 2020. These models underwent 4,000 update steps, with a batch size of 8 and a learning rate of 0.0008. It is important to note that some parameters, such as the warm-up steps and the optimizer, were consistent throughout the pretraining and fine-tuning stages. This consistency supported a cohesive approach to model development. Moreover, during fine-tuning for BA prediction, we consciously limited hyperparameter tuning, which helps avoid overfitting and ensures the effectiveness of mutation scanning.

# Supplementary Notes

The PDBbind database is a widely used benchmark for evaluating protein-ligand binding affinities. The core sets from CASF-2007, CASF-2013, and CASF-2016 are commonly employed for validation purposes. However, different studies have used various training sets to develop prediction models. The CASF benchmarks provide the refined set as a standard training dataset to ensure fair comparisons across models. Notably, many previous studies have used the refined set for training and demonstrated impressive accuracy in binding affinity prediction. However, the

performance of these models when trained on larger datasets, such as the general set, remains unclear. This raises questions about their scalability and effectiveness when applied to more diverse protein-ligand complexes.

In this work, the primary goal is to develop a robust predictor for binding affinity, especially for new protein-ligand complexes, such as the Mpro-nirmatrelvir complex and its mutated variants. To achieve this, we utilized a larger training dataset, specifically the general set, to ensure the highest accuracy in binding affinity prediction. Table 1 in the main text highlights recent models trained on the larger general set. For a transparent overview of previous models, Table S8 below presents the binding affinity prediction performance on the PDBbind core sets for models trained on the refined set.

Table S8: Performance of previous models on CASF benchmark datasets[a]

| Model | CASF-2007 | CASF-2013 | CASF-2016 | PDBbind 2016 |
|---|---|---|---|---|
| Training size | 1105 | 2764 | 3772 | 3767 |
| Testing size | 195 | 195 | 285 | 290 |
| PerSpect[S58] | 0.836 (1.847) | 0.793 (1.956) | | 0.840 (1.724) |
| TopBP[S50] | 0.827 (1.93) | 0.808 (1.95) | | 0.861 (1.65) |
| AGL-score[S59] | 0.83 (1.864) | 0.792 (1.973) | 0.833 (1.733) | |
| DC-GBT[S60] | 0.824 (1.911) | 0.799 (1.952) | | 0.843 (1.711) |
| OPRC[S61] | 0.821 (1.926) | 0.789 (2.010) | | 0.838 (1.736) |
| PLEC[S62] | | 0.757 (2.006) | | 0.817 (SD=1.712) |
| Pancy[S63] | | 0.70 (2.194) | | 0.78 (1.931) |
| ChemPLP@GOLD[S64] | | 0.579 (2.991) | | 0.614 |
| PMH-Transformer[S65] | 0.837 (1.907) | 0.807 (1.982) | | 0.851(1.701) |
| $\Delta_{vina}$RF[S66] | 0.732 | 0.686 | | 0.816 |
| OnionNet[S67] | | 0.782 (2.049) | | 0.816 (1.742) |
| EISA-score[S68] | 0.825 (1.941) | 0.756 (2.113) | 0.821 (1.835) | |
| PotentialNet[S69] | 0.822 (SD=1.892) | | | |
| X-Score::HM[S64] | 0.649 | 0.614 (2.421) | | 0.609 |
| RF::VinaElem[S70] | 0.803 (1.935) | | | |
| KDeep[S71] | | | | 0.82 (1.731) |

[a]The PCC and RMSE (in parentheses, in the unit kcal/mol) for all methods are provided. The refined set of each (year) version of PDBbind[S64,S72–S74] was used as the training set. [b]The CASF-2016 dataset plus five additional protein-ligand complexes (also known as the PDBbind 2016 core set).

# References


(S1) Hu, Y.; Lewandowski, E. M.; Tan, H.; Zhang, X.; Morgan, R. T.; Zhang, X.; Jacobs, L. M.; Butler, S. G.; Gongora, M. V.; Choy, J.; others Naturally occurring mutations of SARS-

CoV-2 main protease confer drug resistance to nirmatrelvir. *ACS Central Science* **2023**, *9*, 1658–1669.

(S2) Hoffman, R. L.; Kania, R. S.; Brothers, M. A.; Davies, J. F.; Ferre, R. A.; Gajiwala, K. S.; He, M.; Hogan, R. J.; Kozminski, K.; Li, L. Y.; others Discovery of ketone-based covalent inhibitors of coronavirus 3CL proteases for the potential therapeutic treatment of COVID-19. *Journal of medicinal chemistry* **2020**, *63*, 12725–12747.

(S3) Lee, C.-C.; Kuo, C.-J.; Ko, T.-P.; Hsu, M.-F.; Tsui, Y.-C.; Chang, S.-C.; Yang, S.; Chen, S.-J.; Chen, H.-C.; Hsu, M.-C.; others Structural basis of inhibition specificities of 3C and 3C-like proteases by zinc-coordinating and peptidomimetic compounds. *Journal of Biological Chemistry* **2009**, *284*, 7646–7655.

(S4) Dai, W.; Zhang, B.; Jiang, X.-M.; Su, H.; Li, J.; Zhao, Y.; Xie, X.; Jin, Z.; Peng, J.; Liu, F.; others Structure-based design of antiviral drug candidates targeting the SARS-CoV-2 main protease. *Science* **2020**, *368*, 1331–1335.

(S5) Lee, C.-C.; Kuo, C.-J.; Hsu, M.-F.; Liang, P.-H.; Fang, J.-M.; Shie, J.-J.; Wang, A. H.-J. Structural basis of mercury-and zinc-conjugated complexes as SARS-CoV 3C-like protease inhibitors. *FEBS letters* **2007**, *581*, 5454–5458.

(S6) Yang, S.; Chen, S.-J.; Hsu, M.-F.; Wu, J.-D.; Tseng, C.-T. K.; Liu, Y.-F.; Chen, H.-C.; Kuo, C.-W.; Wu, C.-S.; Chang, L.-W.; others Synthesis, crystal structure, structure-activity relationships, and antiviral activity of a potent SARS coronavirus 3CL protease inhibitor. *Journal of medicinal chemistry* **2006**, *49*, 4971–4980.

(S7) Zhang, L.; Lin, D.; Kusov, Y.; Nian, Y.; Ma, Q.; Wang, J.; Von Brunn, A.; Leyssen, P.; Lanko, K.; Neyts, J.; others $\alpha$-Ketoamides as broad-spectrum inhibitors of coronavirus and enterovirus replication: structure-based design, synthesis, and activity assessment. *Journal of medicinal chemistry* **2020**, *63*, 4562–4578.

(S8) Lu, I.-L.; Mahindroo, N.; Liang, P.-H.; Peng, Y.-H.; Kuo, C.-J.; Tsai, K.-C.; Hsieh, H.-P.; Chao, Y.-S.; Wu, S.-Y. Structure-based drug design and structural biology study of novel nonpeptide inhibitors of severe acute respiratory syndrome coronavirus main protease. *Journal of medicinal chemistry* **2006**, *49*, 5154–5161.

(S9) Vuong, W.; Khan, M. B.; Fischer, C.; Arutyunova, E.; Lamer, T.; Shields, J.; Saffran, H. A.; McKay, R. T.; van Belkum, M. J.; Joyce, M. A.; others Feline coronavirus drug inhibits the main protease of SARS-CoV-2 and blocks virus replication. *Nature communications* **2020**, *11*, 4282.

(S10) Bacha, U.; Barrila, J.; Gabelli, S. B.; Kiso, Y.; Mario Amzel, L.; Freire, E. Development of broad-spectrum halomethyl ketone inhibitors against coronavirus main protease 3CLpro. *Chemical biology & drug design* **2008**, *72*, 34–49.

(S11) Rathnayake, A. D.; Zheng, J.; Kim, Y.; Perera, K. D.; Mackin, S.; Meyerholz, D. K.; Kashipathy, M. M.; Battaile, K. P.; Lovell, S.; Perlman, S.; others 3C-like protease inhibitors block coronavirus replication in vitro and improve survival in MERS-CoV–infected mice. *Science translational medicine* **2020**, *12*, eabc5332.

(S12) Sacco, M. D.; Ma, C.; Lagarias, P.; Gao, A.; Townsend, J. A.; Meng, X.; Dube, P.; Zhang, X.; Hu, Y.; Kitamura, N.; others Structure and inhibition of the SARS-CoV-2 main protease reveal strategy for developing dual inhibitors against Mpro and cathepsin L. *Science Advances* **2020**, *6*, eabe0751.

(S13) Wang, H.; He, S.; Deng, W.; Zhang, Y.; Li, G.; Sun, J.; Zhao, W.; Guo, Y.; Yin, Z.; Li, D.; others Comprehensive insights into the catalytic mechanism of middle east respiratory syndrome 3C-like protease and severe acute respiratory syndrome 3C-like protease. *ACS catalysis* **2020**, *10*, 5871–5890.

(S14) Zhang, L.; Lin, D.; Sun, X.; Curth, U.; Drosten, C.; Sauerhering, L.; Becker, S.; Rox, K.;

Hilgenfeld, R. Crystal structure of SARS-CoV-2 main protease provides a basis for design of improved $\alpha$-ketoamide inhibitors. *Science* **2020**, *368*, 409–412.

(S15) Su, H.-x.; Yao, S.; Zhao, W.-f.; Li, M.-j.; Liu, J.; Shang, W.-j.; Xie, H.; Ke, C.-q.; Hu, H.-c.; Gao, M.-n.; others Anti-SARS-CoV-2 activities in vitro of Shuanghuanglian preparations and bioactive ingredients. *Acta Pharmacologica Sinica* **2020**, *41*, 1167–1177.

(S16) Verschueren, K. H.; Pumpor, K.; Anemüller, S.; Chen, S.; Mesters, J. R.; Hilgenfeld, R. A structural view of the inactivation of the SARS coronavirus main proteinase by benzotriazole esters. *Chemistry & Biology* **2008**, *15*, 597–606.

(S17) Goetz, D.; Choe, Y.; Hansell, E.; Chen, Y.; McDowell, M.; Jonsson, C.; Roush, W.; McKerrow, J.; Craik, C. Substrate specificity profiling and identification of a new class of inhibitor for the major protease of the SARS coronavirus. *Biochemistry* **2007**, *46*, 8744–8752.

(S18) Zhu, L.; George, S.; Schmidt, M. F.; Al-Gharabli, S. I.; Rademann, J.; Hilgenfeld, R. Peptide aldehyde inhibitors challenge the substrate specificity of the SARS-coronavirus main protease. *Antiviral research* **2011**, *92*, 204–212.

(S19) Turlington, M.; Chun, A.; Tomar, S.; Eggler, A.; Grum-Tokars, V.; Jacobs, J.; Daniels, J. S.; Dawson, E.; Saldanha, A.; Chase, P.; others Discovery of N-(benzo [1, 2, 3] triazol-1-yl)-N-(benzyl) acetamido) phenyl) carboxamides as severe acute respiratory syndrome coronavirus (SARS-CoV) 3CLpro inhibitors: identification of ML300 and noncovalent nanomolar inhibitors with an induced-fit binding. *Bioorganic & medicinal chemistry letters* **2013**, *23*, 6172–6177.

(S20) Yang, H.; Xie, W.; Xue, X.; Yang, K.; Ma, J.; Liang, W.; Zhao, Q.; Zhou, Z.; Pei, D.; Ziebuhr, J.; others Design of wide-spectrum inhibitors targeting coronavirus main proteases. *PLoS biology* **2005**, *3*, e324.

(S21) Chuck, C.-P.; Chen, C.; Ke, Z.; Wan, D. C.-C.; Chow, H.-F.; Wong, K.-B. Design, synthesis and crystallographic analysis of nitrile-based broad-spectrum peptidomimetic inhibitors for coronavirus 3C-like proteases. *European journal of medicinal chemistry* **2013**, *59*, 1–6.

(S22) Shimamoto, Y.; Hattori, Y.; Kobayashi, K.; Teruya, K.; Sanjoh, A.; Nakagawa, A.; Yamashita, E.; Akaji, K. Fused-ring structure of decahydroisoquinolin as a novel scaffold for SARS 3CL protease inhibitors. *Bioorganic & medicinal chemistry* **2015**, *23*, 876–890.

(S23) Ghosh, A. K.; Xi, K.; Ratia, K.; Santarsiero, B. D.; Fu, W.; Harcourt, B. H.; Rota, P. A.; Baker, S. C.; Johnson, M. E.; Mesecar, A. D. Design and synthesis of peptidomimetic severe acute respiratory syndrome chymotrypsin-like protease inhibitors. *Journal of medicinal chemistry* **2005**, *48*, 6767–6771.

(S24) Ghosh, A. K.; Xi, K.; Grum-Tokars, V.; Xu, X.; Ratia, K.; Fu, W.; Houser, K. V.; Baker, S. C.; Johnson, M. E.; Mesecar, A. D. Structure-based design, synthesis, and biological evaluation of peptidomimetic SARS-CoV 3CLpro inhibitors. *Bioorganic & medicinal chemistry letters* **2007**, *17*, 5876–5880.

(S25) Nguyen, D. D.; Gao, K.; Chen, J.; Wang, R.; Wei, G.-W. Unveiling the molecular mechanism of SARS-CoV-2 main protease inhibition from 137 crystal structures using algebraic topology and deep learning. *Chemical science* **2020**, *11*, 12036–12046.

(S26) Clayton, J.; de Oliveira, V. M.; Ibrahim, M. F.; Sun, X.; Mahinthichaichan, P.; Shen, M.; Hilgenfeld, R.; Shen, J. Integrative Approach to Dissect the Drug Resistance Mechanism of the H172Y Mutation of SARS-CoV-2 Main Protease. *Journal of Chemical Information and Modeling* **2023**,

(S27) Iketani, S.; Mohri, H.; Culbertson, B.; Hong, S. J.; Duan, Y.; Luck, M. I.; Annavajhala, M. K.; Guo, Y.; Sheng, Z.; Uhlemann, A.-C.; others Multiple pathways for SARS-CoV-2 resistance to nirmatrelvir. *Nature* **2023**, *613*, 558–564.

(S28) Cang, Z.; Wei, G.-W. TopologyNet: Topology based deep convolutional and multi-task neural networks for biomolecular property predictions. *PLoS computational biology* **2017**, *13*, e1005690.

(S29) Zomorodian, A.; Carlsson, G. Computing persistent homology. Proceedings of the twentieth annual symposium on Computational geometry. 2004; pp 347–356.

(S30) Edelsbrunner; Letscher; Zomorodian Topological persistence and simplification. *Discrete & Computational Geometry* **2002**, *28*, 511–533.

(S31) Wasserman, L. Topological data analysis. *Annual Review of Statistics and Its Application* **2018**, *5*, 501–532.

(S32) Townsend, J.; Micucci, C. P.; Hymel, J. H.; Maroulas, V.; Vogiatzis, K. D. Representation of molecular structures with persistent homology for machine learning applications in chemistry. *Nature communications* **2020**, *11*, 3230.

(S33) Nguyen, D. D.; Cang, Z.; Wu, K.; Wang, M.; Cao, Y.; Wei, G.-W. Mathematical deep learning for pose and binding affinity prediction and ranking in D3R Grand Challenges. *Journal of computer-aided molecular design* **2019**, *33*, 71–82.

(S34) Nguyen, D. D.; Gao, K.; Wang, M.; Wei, G.-W. MathDL: mathematical deep learning for D3R Grand Challenge 4. *Journal of computer-aided molecular design* **2020**, *34*, 131–147.

(S35) Papamarkou, T.; Birdal, T.; Bronstein, M. M.; Carlsson, G. E.; Curry, J.; Gao, Y.; Hajij, M.; Kwitt, R.; Lio, P.; Di Lorenzo, P.; others Position: Topological Deep Learning is the New Frontier for Relational Learning. Forty-first International Conference on Machine Learning. 2024.

(S36) Wei, X.; Wei, G.-W. Persistent Topological Laplacians–a Survey. *arXiv preprint arXiv:2312.07563* **2023**,

(S37) Wang, R.; Nguyen, D. D.; Wei, G.-W. Persistent spectral graph. *International journal for numerical methods in biomedical engineering* **2020**, *36*, e3376.

(S38) Chen, J.; Zhao, R.; Tong, Y.; Wei, G.-W. Evolutionary de rham-hodge method. *Discrete and continuous dynamical systems. Series B* **2021**, *26*, 3785.

(S39) Jones, B.; Wei, G. Persistent Directed Flag Laplacian. *Foundations of Data Science* **doi: 10.3934/fods.2024048, 2024**,

(S40) Wei, X.; Wei, G.-W. Persistent sheaf laplacians. *Foundations of Data Science, doi: 10.3934/fods.2024033* **2024**,

(S41) Wang, R.; Wei, G.-W. Persistent path laplacian. *Foundations of data science (Springfield, Mo.)* **2023**, *5*, 26.

(S42) Chen, D.; Liu, J.; Wu, J.; Wei, G.-W.; Pan, F.; Yau, S.-T. Path topology in molecular and materials sciences. *The Journal of Physical Chemistry Letters* **2023**, *14*, 954–964.

(S43) Liu, X.; Feng, H.; Wu, J.; Xia, K. Persistent spectral hypergraph based machine learning (PSH-ML) for protein-ligand binding affinity prediction. *Briefings in Bioinformatics* **2021**, *22*, bbab127.

(S44) Chen, D.; Liu, J.; Wu, J.; Wei, G.-W. Persistent hyperdigraph homology and persistent hyperdigraph Laplacians. *Foundations of Data Science* **2023**, *5*, 558–588.

(S45) Horak, D.; Jost, J. Spectra of combinatorial Laplace operators on simplicial complexes. *Advances in Mathematics* **2013**, *244*, 303–336.

(S46) Eckmann, B. Harmonische funktionen und randwertaufgaben in einem komplex. *Commentarii Mathematici Helvetici* **1944**, *17*, 240–255.

(S47) Chen, J.; Zhao, R.; Tong, Y.; Wei, G.-W. Evolutionary de Rham-Hodge method. *arXiv preprint arXiv:1912.12388* **2019**,

(S48) Mémoli, F.; Wan, Z.; Wang, Y. Persistent Laplacians: Properties, algorithms and implications. *SIAM Journal on Mathematics of Data Science* **2022**, *4*, 858–884.

(S49) Liu, J.; Li, J.; Wu, J. The algebraic stability for persistent Laplacians. *arXiv preprint arXiv:2302.03902* **2023**,

(S50) Cang, Z.; Mu, L.; Wei, G.-W. Representability of algebraic topology for biomolecules in machine learning based scoring and virtual screening. *PLoS computational biology* **2018**, *14*, e1005929.

(S51) Kozlov, D. *Combinatorial algebraic topology*; Springer Science & Business Media, 2008; Vol. 21.

(S52) Lovász, L. Kneser's conjecture, chromatic number, and homotopy. *Journal of Combinatorial Theory, Series A* **1978**, *25*, 319–324.

(S53) He, K.; Chen, X.; Xie, S.; Li, Y.; Dollár, P.; Girshick, R. Masked autoencoders are scalable vision learners. Proceedings of the IEEE/CVF conference on computer vision and pattern recognition. 2022; pp 16000–16009.

(S54) Rives, A.; Meier, J.; Sercu, T.; Goyal, S.; Lin, Z.; Liu, J.; Guo, D.; Ott, M.; Zitnick, C. L.; Ma, J.; others Biological structure and function emerge from scaling unsupervised learning to 250 million protein sequences. *Proceedings of the National Academy of Sciences* **2021**, *118*, e2016239118.

(S55) Chen, D.; Zheng, J.; Wei, G.-W.; Pan, F. Extracting predictive representations from hundreds of millions of molecules. *The journal of physical chemistry letters* **2021**, *12*, 10793–10801.

(S56) Pedregosa, F.; Varoquaux, G.; Gramfort, A.; Michel, V.; Thirion, B.; Grisel, O.; Blondel, M.; Prettenhofer, P.; Weiss, R.; Dubourg, V.; others Scikit-learn: Machine learning in Python. *the Journal of machine Learning research* **2011**, *12*, 2825–2830.

(S57) Ke, G.; Meng, Q.; Finley, T.; Wang, T.; Chen, W.; Ma, W.; Ye, Q.; Liu, T.-Y. Lightgbm: A highly efficient gradient boosting decision tree. *Advances in neural information processing systems* **2017**, *30*.

(S58) Meng, Z.; Xia, K. Persistent spectral–based machine learning (PerSpect ML) for protein-ligand binding affinity prediction. *Science advances* **2021**, *7*, eabc5329.

(S59) Nguyen, D. D.; Wei, G.-W. AGL-score: algebraic graph learning score for protein–ligand binding scoring, ranking, docking, and screening. *Journal of chemical information and modeling* **2019**, *59*, 3291–3304.

(S60) Liu, X.; Feng, H.; Wu, J.; Xia, K. Dowker complex based machine learning (DCML) models for protein-ligand binding affinity prediction. *PLoS computational biology* **2022**, *18*, e1009943.

(S61) Wee, J.; Xia, K. Ollivier persistent Ricci curvature-based machine learning for the protein–ligand binding affinity prediction. *Journal of Chemical Information and Modeling* **2021**, *61*, 1617–1626.

(S62) Wójcikowski, M.; Kukiełka, M.; Stepniewska-Dziubinska, M. M.; Siedlecki, P. Development of a protein–ligand extended connectivity (PLEC) fingerprint and its application for binding affinity predictions. *Bioinformatics* **2019**, *35*, 1334–1341.

(S63) Stepniewska-Dziubinska, M. M.; Zielenkiewicz, P.; Siedlecki, P. Development and evaluation of a deep learning model for protein–ligand binding affinity prediction. *Bioinformatics* **2018**, *34*, 3666–3674.

(S64) Su, M.; Yang, Q.; Du, Y.; Feng, G.; Liu, Z.; Li, Y.; Wang, R. Comparative assessment of scoring functions: the CASF-2016 update. *Journal of chemical information and modeling* **2018**, *59*, 895–913.

(S65) Feng, H.; Shen, L.; Liu, J.; Wei, G.-W. Mayer-homology learning prediction of protein-ligand binding affinities. *arXiv preprint arXiv:2408.13299* **2024**,

(S66) Wang, C.; Zhang, Y. Improving scoring-docking-screening powers of protein–ligand scoring functions using random forest. *Journal of computational chemistry* **2017**, *38*, 169–177.

(S67) Zheng, L.; Fan, J.; Mu, Y. Onionnet: a multiple-layer intermolecular-contact-based convolutional neural network for protein–ligand binding affinity prediction. *ACS omega* **2019**, *4*, 15956–15965.

(S68) Rana, M. M.; Nguyen, D. D. EISA-Score: Element Interactive Surface Area score for protein–ligand binding affinity prediction. *Journal of Chemical Information and Modeling* **2022**, *62*, 4329–4341.

(S69) Feinberg, E. N.; Sur, D.; Wu, Z.; Husic, B. E.; Mai, H.; Li, Y.; Sun, S.; Yang, J.; Ramsundar, B.; Pande, V. S. PotentialNet for molecular property prediction. *ACS central science* **2018**, *4*, 1520–1530.

(S70) Li, H.; Leung, K.-S.; Wong, M.-H.; Ballester, P. J. Improving AutoDock Vina using random forest: the growing accuracy of binding affinity prediction by the effective exploitation of larger data sets. *Molecular informatics* **2015**, *34*, 115–126.

(S71) Jiménez, J.; Skalic, M.; Martinez-Rosell, G.; De Fabritiis, G. K deep: protein–ligand absolute binding affinity prediction via 3d-convolutional neural networks. *Journal of chemical information and modeling* **2018**, *58*, 287–296.

(S72) Liu, Z.; Li, Y.; Han, L.; Li, J.; Liu, J.; Zhao, Z.; Nie, W.; Liu, Y.; Wang, R. PDB-wide collection of binding data: current status of the PDBbind database. *Bioinformatics* **2015**, *31*, 405–412.

(S73) Cheng, T.; Li, X.; Li, Y.; Liu, Z.; Wang, R. Comparative assessment of scoring functions on a diverse test set. *Journal of chemical information and modeling* **2009**, *49*, 1079–1093.

(S74) Li, Y.; Han, L.; Liu, Z.; Wang, R. Comparative assessment of scoring functions on an updated benchmark: 2. Evaluation methods and general results. *Journal of chemical information and modeling* **2014**, *54*, 1717–1736.
